# Supplementary material for: Quantifying the effect of phenotype on clustering behaviour in melanoma: from monoculture to co-culture
Source: arXiv:2604.24673 source file (2026-09-05)
Supplement: Supplementary file 1 [file supplementary-information.tex]

\documentclass[pdflatex,sn-basic]{sn-jnl} 
\usepackage{graphicx}%
\usepackage{multirow}%
\usepackage{amsmath,amssymb,amsfonts}%
\usepackage{amsthm}%
\usepackage{mathrsfs}%
\usepackage[title]{appendix}%
\usepackage{xcolor}%
\usepackage{textcomp}%
\usepackage{manyfoot}%
\usepackage{booktabs}%
\usepackage{algorithm}%
\usepackage{algorithmicx}%
\usepackage{algpseudocode}%
\usepackage{listings}%
\usepackage{mathtools}

% Enforce S-numbering

\begin{document}

\title{Supplementary Information for:
\emph{Quantifying the effect of phenotype on clustering behaviour in melanoma: from monoculture to co-culture}}

\author*[1,2]{\fnm{Nathan} \sur{Schofield}}\email{nathan.schofield@dtc.ox.ac.uk}

\author[2]{\fnm{Richard} \sur{White}}\email{richard.white@ludwig.ox.ac.uk}
% \equalcont{These authors contributed equally to this work.}
% \equalcont{These authors contributed equally to this work.}

\author[1]{\fnm{Ruth} \sur{Baker}}\email{ruth.baker@maths.ox.ac.uk}

\author[1,2]{\fnm{Helen} \sur{Byrne}}\email{helen.byrne@maths.ox.ac.uk}

\affil[1]{\orgdiv{Mathematical Institute}, 
    \orgname{University of Oxford}, 
    \orgaddress{
        \street{Andrew Wiles Building, Woodstock Road}, 
        \city{Oxford}, 
        \postcode{OX2 6GG}, 
        \state{England}, 
        \country{United Kingdom}}}
\affil[2]{\orgdiv{Ludwig Institute for Cancer Research}, 
    \orgname{University of Oxford}, 
    \orgaddress{
        \street{Old Road Campus Research Building, Roosevelt Drive}, 
        \city{Oxford}, 
        \postcode{OX3 7DQ}, 
        \state{England}, 
        \country{United Kingdom}}}

\maketitle

\section{Data and image analysis\label{section:ImAnalysis}}

Throughout this paper we have analysed previously published data \citep{campbell_cooperation_2021} generated from two melanoma cell phenotypes of the ZMEL1 line \citep{heilmann_quantitative_2015}. In this section, we describe in more detail the biological data and explain how we converted it into cluster size distributions and summary statistics that were then used to motivate and calibrate the variants of the mathematical model.

\bigskip
\noindent\textbf{Homogeneous \textit{in vitro} experiments}

Homogeneous populations of proliferative and invasive cells were tagged with green fluorescent protein (GFP) \citep{tsien_green_1998}. Individual cells (clusters of size one) were added to culture medium in a three-dimensional well, with two experimental repeats for each phenotype. The dynamics of the spherical clusters were observed over a 72-hour period. 
Maximum intensity projection images, showing two-dimensional representations of the three-dimensional wells were taken every 30 minutes (for further details see \citep{campbell_cooperation_2021}).

\bigskip
\noindent\textbf{Heterogeneous \textit{in vitro} experiments}

A second dataset was generated by co-culturing proliferative and invasive cells in a 1:1 ratio over a period of 72 hours. Both phenotypes were tagged with GFP, and proliferative cells were additionally tagged with tdTomato (a red fluorescent protein) \citep{shaner_improved_2004}. Maximum intensity projection images were taken every 30 minutes, which allows us to observe the locations of cells in the well irrespective of their phenotype. However, because these are two-dimensional projections of a three-dimensional environment, the apparent spatial arrangement of phenotypes within a cluster depends on the viewing angle. Rotating the cluster in three-dimensions would change the projection, so we cannot reliably infer the phenotypic composition of individual clusters from these images.

\vspace{1em}
\noindent \textbf{Image analysis \label{section:ImAnalysisPipeline}}

The image analysis techniques described in Figure \ref{fig:RAW_images}A were used to extract dynamic data relating to cluster size distributions from each experiment. First, we applied a binary mask using the Otsu automatic image thresholding method \citep{otsu_threshold_1979} (see Figure \ref{fig:RAW_images}B). The thresholding value \citep{otsu_threshold_1979} was chosen to minimise the intra-class variance between the background and object pixel classes. The Otsu method is widely used for binary classification of imaging data \citep{davies_chapter_2018, lu_chapter_2024, padmasini_chapter_2018}, and is among the most popular techniques for optimal thresholding \citep{gonzales-barron_comparison_2006, nixon_basic_2012}. The locations and sizes of all clusters were recorded, and the distributions of cluster sizes averaged over both experimental repeats. The evolution and ancestry of each cluster were also tracked, focusing on coagulation events where two or more clusters merge to form a larger cluster, and fragmentation events where a cluster splits into two or more smaller clusters.

\begin{figure}[]
    \centering
    \includegraphics[width=\textwidth]{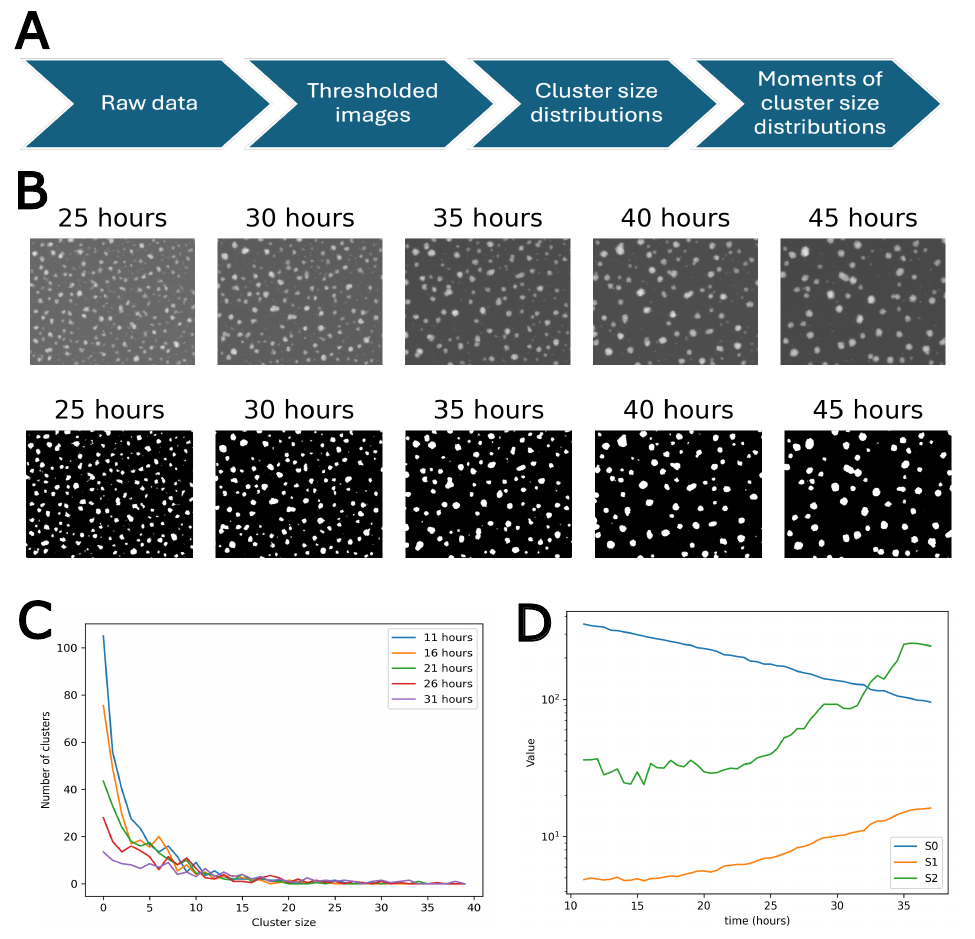}
    \caption{Schematic for converting biological imaging data into quantitative inputs for the mathematical models. invasive cell monoculture experiment. (A) Pipeline schematic. (B) Visualisation of the raw data (upper row) and the associated, thresholded data (lower row) during the course of an experiment. (C) Cluster size distributions. (D) Summary statistics generated from cluster size distributions.}
    \label{fig:RAW_images}
\end{figure}

In Figure \ref{fig:RAW_images}B (top row) we present typical images from the invasive cell experiments. At early timepoints, there are a large number of small clusters whereas at later times the cells form a small number of larger clusters (see Figure \ref{fig:RAW_images}C). 
To reduce the number of noise parameters needed to fit mathematical models to the data, %by giving a lower dimensional representation of the data, 
we compute summary statistics ($S_h$, $h=0,1,2$) of the distributions (see Figure \ref{fig:RAW_images}D).

\subsubsection*{Justification of modelling assumptions} 

\begin{figure}[H]
\centering
\includegraphics[width=\textwidth]{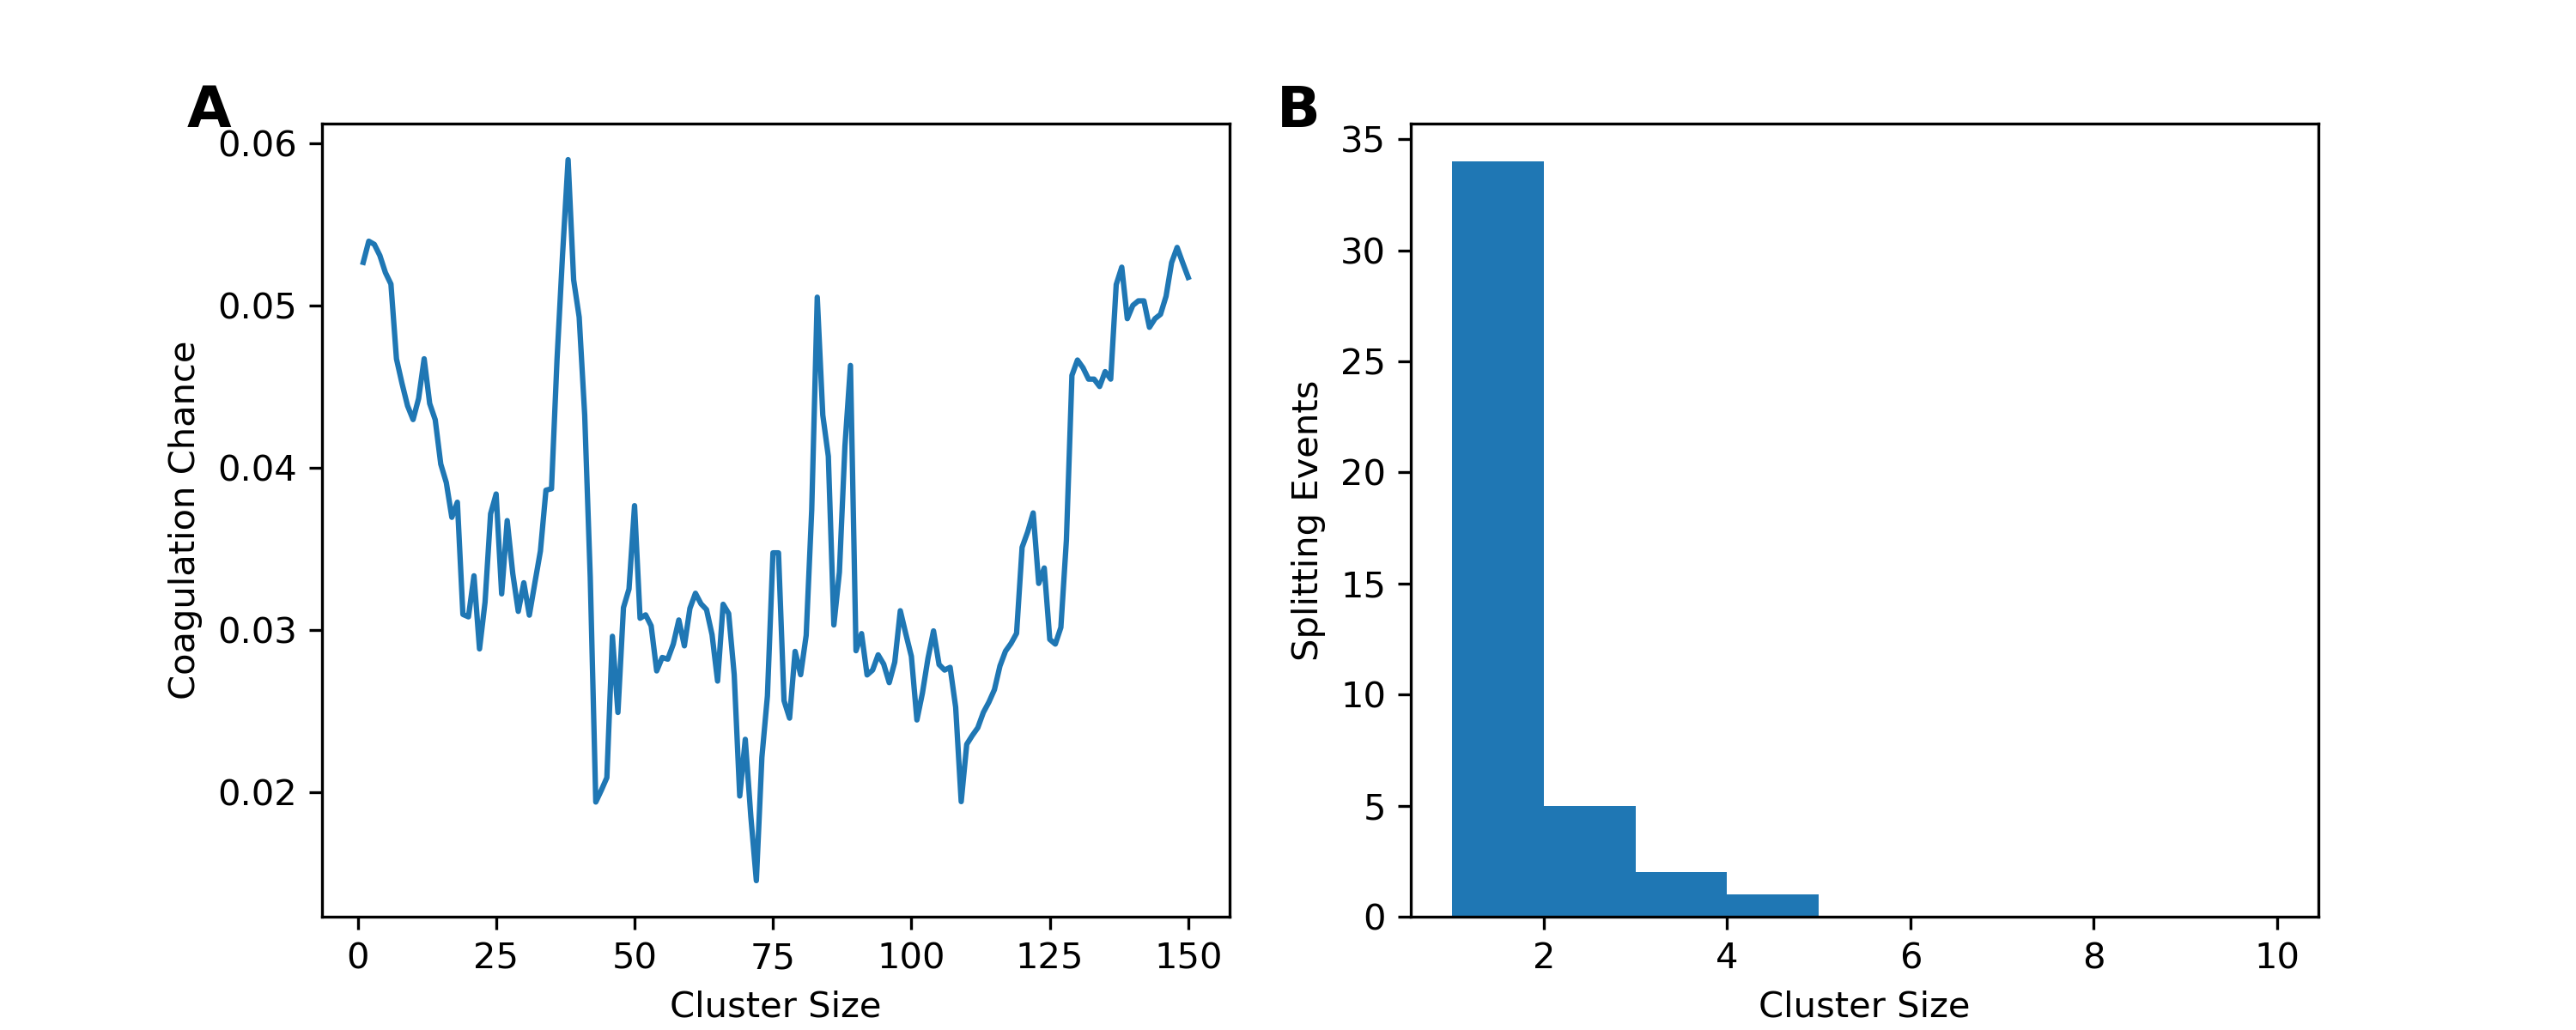}
\caption{(A) Probability of coagulation as a function of cluster size in invasive cell monoculture experiments. The data supports the assumption of a constant coagulation kernel. (B) Distribution of cluster sizes resulting from fragmentation events in invasive cell experiments.}
\label{fig:model-motivation}
\end{figure}

Figure \ref{fig:model-motivation}A quantifies the likelihood of coagulation events across different cluster sizes in invasive cell monoculture experiments. We observe a lack of a clear trend in the chance of coagulation as cluster sizes change which justifies the modelling assumption of a constant coagulation rate in the ordinary differential equation (ODE) framework.
Figure \ref{fig:model-motivation}B illustrates the distribution of cluster sizes produced by fragmentation events observed in co-cultured experiments. We see that clusters do not split into clusters of similar size. Instead, a small cluster, generally of size one, detaches from the larger cluster. This leads to the distribution in Figure \ref{fig:model-motivation}B where most fragmentation events create a cluster of size one. These observations motivate the inclusion of shedding as the particular form of fragmentation in the model.

\section{Heterogeneous model \label{section:HeteroMathModel}}

\textbf{Model derivation}

The model in Section 2.2 can be extended to describe heterogeneous clusters in a natural way, by considering the cluster size and its phenotypic composition (that is, the number of cells of each phenotype within a given cluster). We assume that each cluster consists of two melanoma cell phenotypes (proliferative and invasive cells). We denote by $\Phi_{i,k}(t)$ the number of clusters containing a total of $i\geq 1$ cells, with $k$ proliferative cells, $0 \leq k \leq i$ (and $i-k$ invasive cells). As for the homogeneous model, the mechanisms driving the time evolution of $\Phi_{i,k}(t)$ are assumed to be cluster coagulation, cell proliferation, and cluster shedding. The model is formulated as a system of ODEs of the form:

\begin{equation}
\frac{\text{d}\Phi_{i,k}}{\text{d}t} = T_{i,k}^{\text{coag}} + T_{i,k}^{\text{prolif},\alpha_{1,2}} + T_{i,k}^{\text{frag},\beta.}
\label{eqn:Hetero-final}
\end{equation}

\noindent \textbf{Coagulation}

The coagulation term models the merging of two clusters to form a larger one. As before, and for simplicity, we assume that the rate of coagulation is constant and independent of cluster size and composition.
As for the monoculture model the net coagulation rate $T_{i,k}^{\text{coag}}$ for $\Phi_{i,k}$ comprises two terms: a loss term due to the coagulation of clusters with $i$ cells of which $k$ are proliferative cells with other clusters and a source term due to their formation from smaller clusters coagulating. Under this assumption, the coagulation term can be written as

\[
T_{i,k}^{\text{coag}} = -\tilde{b} \sum_{l=1}^{\infty} \sum_{m=0}^{l}  \Phi_{i,k} \Phi_{l,m} + \frac{\tilde{b}}{2} \sum_{u=1}^{i-1} \sum_{v=0}^{\min(u,k)} \Phi_{u,v} \Phi_{i-u,k-v}.
\]

\noindent \textbf{Proliferation}

The proliferation term accounts for the division of cells within clusters, which can increase the cluster size. We introduce two proliferation functions $\tilde{\rho}_1^{\alpha_1}, \tilde{\rho}_2^{\alpha_2}$ which model the proliferation of a proliferative and invasive cell, respectively. The proliferation term $T_{i,k}^{\text{prolif},\alpha_{1,2}}$ for $\Phi_{i,k}$ is defined piecewise to capture different cluster scenarios:

\[
T_{i,k}^{\text{prolif},\alpha_{1,2}} = 
\begin{cases} 
-\tilde{\rho}_{2_{1,0}}^{\alpha_2} \cdot \Phi_{1,0} & \text{if } k = 0 \text{ and } i=0,\\
-\tilde{\rho}_{1_{1,1}}^{\alpha_1} \cdot \Phi_{1,1} & \text{if } k = 1 \text{ and } i=1,\\
-\tilde{\rho}_{2_{i,0}}^{\alpha_2} \cdot \Phi_{i, 0} + \tilde{\rho}_{2_{i-1,0}} ^{\alpha_2}\cdot \Phi_{i-1, 0} & \text{if } k = 0 \text{ and }  i > 1, \\
-(\tilde{\rho}_{1_{i,1}}^{\alpha_1} + \tilde{\rho}_{2_{i,1}}^{\alpha_2}) \cdot \Phi_{i, 1} + \tilde{\rho}_{2_{i-1,1}} \cdot \Phi_{i-1, 1} & \text{if } k = 1 \text{ and }  i > 2, \\
-(\tilde{\rho}_{1_{i,i-1}}^{\alpha_1} + \tilde{\rho}_{2_{i,i-1}}^{\alpha_2}) \cdot \Phi_{i, i-1} + \tilde{\rho}_{1_{i-1,i-2}}^{\alpha_1} \cdot \Phi_{i-1, i-2} & \text{if } k = i-1 \text{ and }  i > 2, \\
-\tilde{\rho}_{1_{i,i}}^{\alpha_1} \cdot \Phi_{i, i} + \tilde{\rho}_{1_{i-1,i-1}}^{\alpha_1} \cdot \Phi_{i-1, i-1} & \text{if } k = i \text{ and }  i > 1, \\
\tilde{\rho}_{2_{Y_{\max}-1,0}}^{\alpha_2}\cdot \Phi_{Y_{\max}-1,0} & \text{if } k = 0 \text{ and } i = Y_{\max},\\
\tilde{\rho}_{2_{Y_{\max}-1,0}}^{\alpha_2}\cdot \Phi_{Y_{\max}-1,0} + \tilde{\rho}_{1_{Y_{\max}-1,Y_{\max}-1}}^{\alpha_1}\cdot \Phi_{Y_{\max}-1,Y_{\max}-1} & \text{if } 0 < k < Y_{\max} \text{ and } i = Y_{\max},\\
\tilde{\rho}_{1_{Y_{\max}-1,Y_{\max}-1}}^{\alpha_1}\cdot \Phi_{Y_{\max}-1,Y_{\max}-1} & \text{if } k = Y_{\max} \text{ and } i = Y_{\max},\\
-(\tilde{\rho}_{1_{i,k}}^{\alpha_1} + \tilde{\rho}_{2_{i,k}}^{\alpha_2}) \cdot \Phi_{i, k} + \tilde{\rho}_{1_{i-1,k-1}}^{\alpha_1} \cdot \Phi_{i-1, k-1} + \tilde{\rho}_{2_{i-1,k}}^{\alpha_2} \cdot \Phi_{i-1, k} & \text{otherwise}.
\end{cases}
\]

\noindent \textbf{Shedding (fragmentation)}

As for the monoculture model, we assume that clusters only shed single cells. Motivated by the experimental data and the results from the analysis of the monoculture model, we assume this shed cell is a proliferative cell. Thus the shedding term $T_{i,k}^{\text{frag},\beta}$ for $\Phi_{i,k}$ is defined as:

\[T_{i,k}^{\text{frag}} = 
\begin{cases} 
+\tilde{\xi}_{2,2}^\beta \Phi_{2,2} + \sum_{u=2}^{\infty}\sum_{v=1}^{u} \tilde{\xi}_{u,v}^\beta \Phi_{u,v} & \text{if } i = 1 \text{ and } k = 1, \\
- \tilde{\xi}_{i,k}^\beta \Phi_{i,k} + \tilde{\xi}_{i+1,k+1}^\beta \Phi_{i+1,k+1} & \text{if } i > 1 \text{ and } k \neq 0, \\
+ \tilde{\xi}_{i+1,1}^\beta \Phi_{i+1,1} & \text{if } k = 0. \\
\end{cases}
\]
\\
The co-culture experiments are initialised with a $1\!:\!1$ ratio of proliferative and invasive cells. If we assume further that there is a total of $\tilde{N}_{\text{TOT}}$ cells at $t=0$ then we close Equation (\ref{eqn:Hetero-final}) by imposing the following initial condition

\begin{equation}
    \Phi_{i,k}(t = 0) = \begin{cases}
        \tilde{N}_{\text{TOT}}/2 \quad &i = 1, k = 1,\\
        \tilde{N}_{\text{TOT}}/2 \quad &i = 1, k = 0,\\
        0 \quad &i > 1.
    \end{cases}
    \label{eqn:Hetero-IC}
\end{equation}

\noindent\textbf{Heterogeneous model parameter identifiability analysis}

We next show how the identifiability of the heterogeneous model parameters depends on the available data.
Figure \ref{fig:Hetero-single-summary-plot} shows that the heterogeneous model is not globally structurally identifiable or practically identifiable without phenotypic composition data. To produce this figure we simulated the heterogeneous model with two different parameter sets. The results in Figure \ref{fig:Hetero-single-summary-plot}A show that when only cluster size distributions are known it is not possible to distinguish between the two parameter sets. Figure \ref{fig:Hetero-single-summary-plot}B-C show that in this case the numbers of cells of each phenotype are distinguishable from one another. These results confirm that the model parameters are not identifiable when only cluster size distributions are known.

\begin{figure}[H]
\centering
\includegraphics[width=\textwidth]{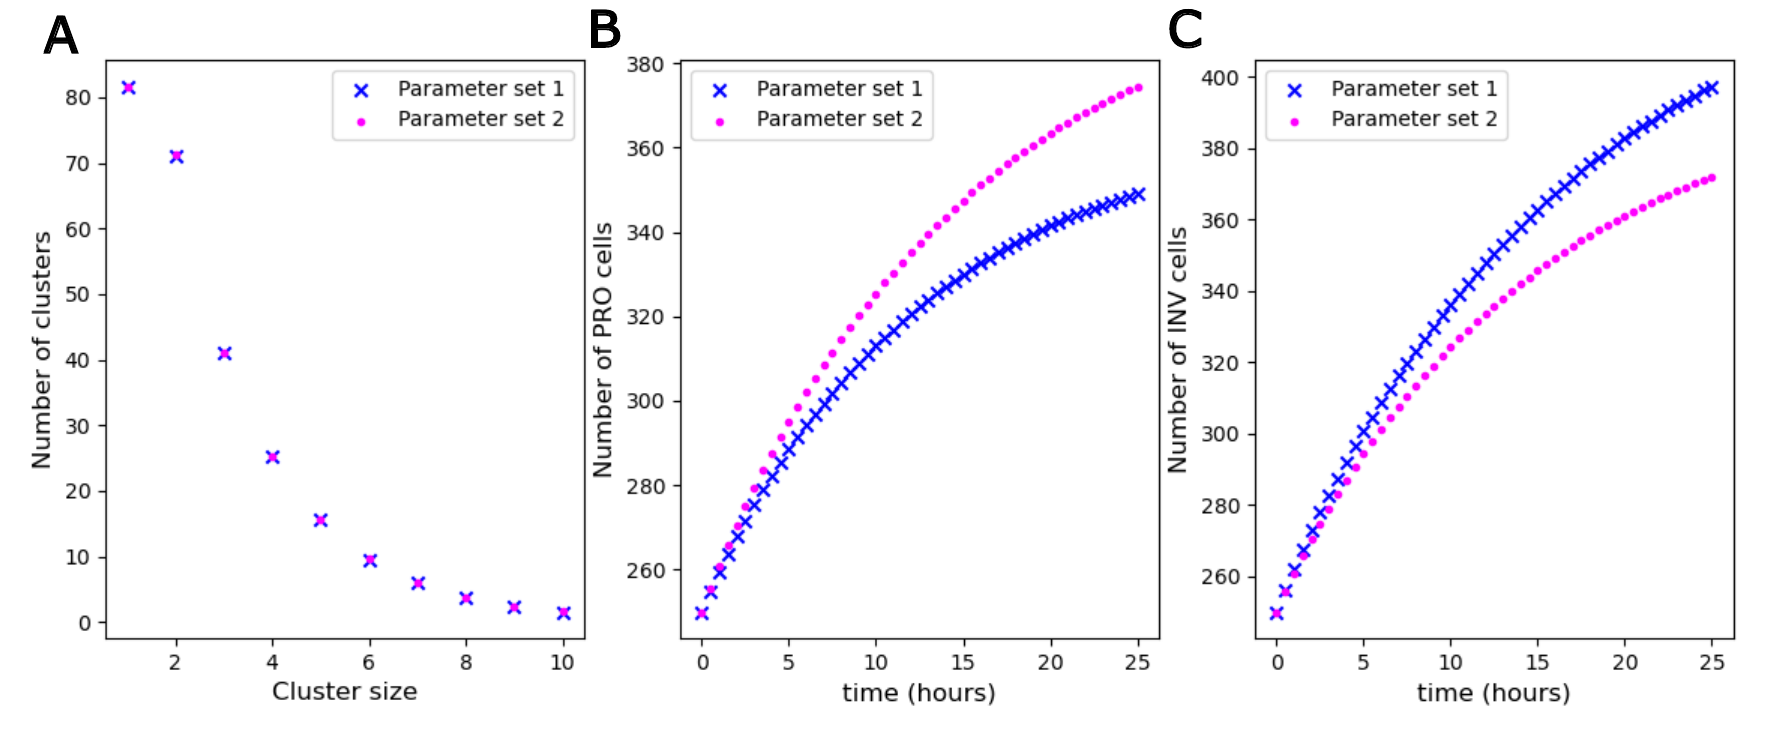}
\caption{Solution plots for a simulation of the heterogeneous model with parameter sets 
$\theta_{1} = \{\tilde{b} = 1.5\times 10^{-4} \,\text{clusters}^{-1}\,\Delta t^{-1}, p_1 = 5 \times 10^{-3} \,\Delta t^{-1}, p_2 = 1 \times 10^{-2} \,\Delta t^{-1}, \tilde{q} = 1 \times 10^{-5} \,\Delta t^{-1}\}$ 
and 
$\theta_{2} = \{\tilde{b} = 1.50\times 10^{-4} \,\text{clusters}^{-1}\,\Delta t^{-1},\, p_1 = 7.69 \times 10^{-3} \,\Delta t^{-1},\, p_2 = 7.41 \times 10^{-3} \,\Delta t^{-1},\, \tilde{q} = 1.00 \times 10^{-4} \,\Delta t^{-1}\}$ with fixed initial condition of $\Phi_{1,0} = 250, \,\Phi_{1,1} = 250, \,\Phi_{i,k}=0$ for $k>1$.
(A) Cluster size distribution at time $(t=30)$. (B) Total number of proliferative cells. (C) Total number of invasive cells.}
\label{fig:Hetero-single-summary-plot}
\end{figure}

\section{Homogeneous model fitted to experimental data \label{section:ExtraPlots}}

We present the results of Bayesian parameter inference applied to experimental data from monocultures of proliferative and invasive melanoma cells, as well as co-cultured populations. Using the homogeneous coagulation--fragmentation--proliferation model framework, we show the marginal and bivariate posterior distributions for the model parameters for two key model variants: $\mathcal{M}_{3,1}$, which includes cell number–dependent proliferation and constant-rate shedding, and $\mathcal{M}_{3,0}$, which also includes cell number–dependent proliferation but neglects shedding.
We only show the results for the model parameters because, as in Figure 1, the noise parameters are not correlated to each other or the parameters in any combination of the $16$ model variants and the different culture conditions (proliferative monoculture, invasive monoculture, or co-cultured). These results in Figures \ref{fig:INV_shed_pairwise}, \ref{fig:PRO_MCMC_plots_cst_shed}, \ref{fig:COMBO_MCMC_plots_cst_shed} relate to model variant $\mathcal{M}_{3,1}$ fitted to the invasive, proliferative, and co-cultured data, respectively; the results in Figures \ref{fig:PRO_MCMC_plots_no_shed}, \ref{fig:INV_MCMC_plots_no_shed}, \ref{fig:COMBO_MCMC_plots_no_shed} relate to model variant $\mathcal{M}_{3,0}$ fitted to the proliferative, invasive, and co-cultured data, respectively.

The posterior distributions highlight key differences between phenotypes and support the conclusions in Section~3.1. In monoculture, invasive phenotype cells exhibit higher coagulation rates, while proliferative phenotype cells show higher proliferation rates. Shedding contributes minimally for invasive phenotype cells and in co-cultures, consistent with the selection of $\mathcal{M}_{3,0}$ as the optimal model in these cases. Co-cultures display hybrid coagulation dynamics resembling both phenotypes, but with proliferation enhanced compared to monocultures.

\begin{table}[]
\centering
\renewcommand{\arraystretch}{1.2}
\resizebox{\textwidth}{!}{%
\begin{tabular}{|c||c|c|c|c|}
\hline
\textbf{Model} $\mathcal{M}_{3,1}$ & $b$ CI $\,(\text{clusters}^{-1}\,\Delta t^{-1})$ & $p$ CI $\,(\Delta t^{-1})$ & $q$ CI $\,(\Delta t^{-1})$ & $N_{\text{TOT}}$ CI \\
\hline
Proliferative cells & $[7.26 \times 10^{-5},\, 7.37 \times 10^{-5}]$ & $[7.10 \times 10^{-3},\, 7.19 \times 10^{-3}]$ & $[2.15 \times 10^{-3},\, 2.41 \times 10^{-3}]$ & $[841,\, 854]$ \\
\hline
Invasive cells & $[1.89 \times 10^{-4},\, 1.99 \times 10^{-4}]$ & $[4.86 \times 10^{-3},\, 5.99 \times 10^{-3}]$ & $[0,\, 5.54 \times 10^{-4}]$ & $[1065,\, 1139]$ \\
\hline
Co-cultured cells & $[1.66 \times 10^{-4},\, 1.70 \times 10^{-4}]$ & $[1.11 \times 10^{-2},\, 1.14 \times 10^{-2}]$ & $[0,\, 1.59 \times 10^{-4}]$ & $[568,\, 582]$ \\
\hline
\end{tabular}
}
\caption{Comparison of the 95\% confidence intervals for MLE values for model parameters $\boldsymbol{\theta}_M = \{b,p,q,N_{\text{TOT}}\}$ across cell lines for model variant $\mathcal{M}_{3,1}$ when fitted to the monocultured proliferative and invasive phenotypic datasets as well as the co-cultured data.}
\label{table:CIs-co-culture-M3,1}
\end{table}

\begin{figure}[H]
\centering
\includegraphics[width=\textwidth]{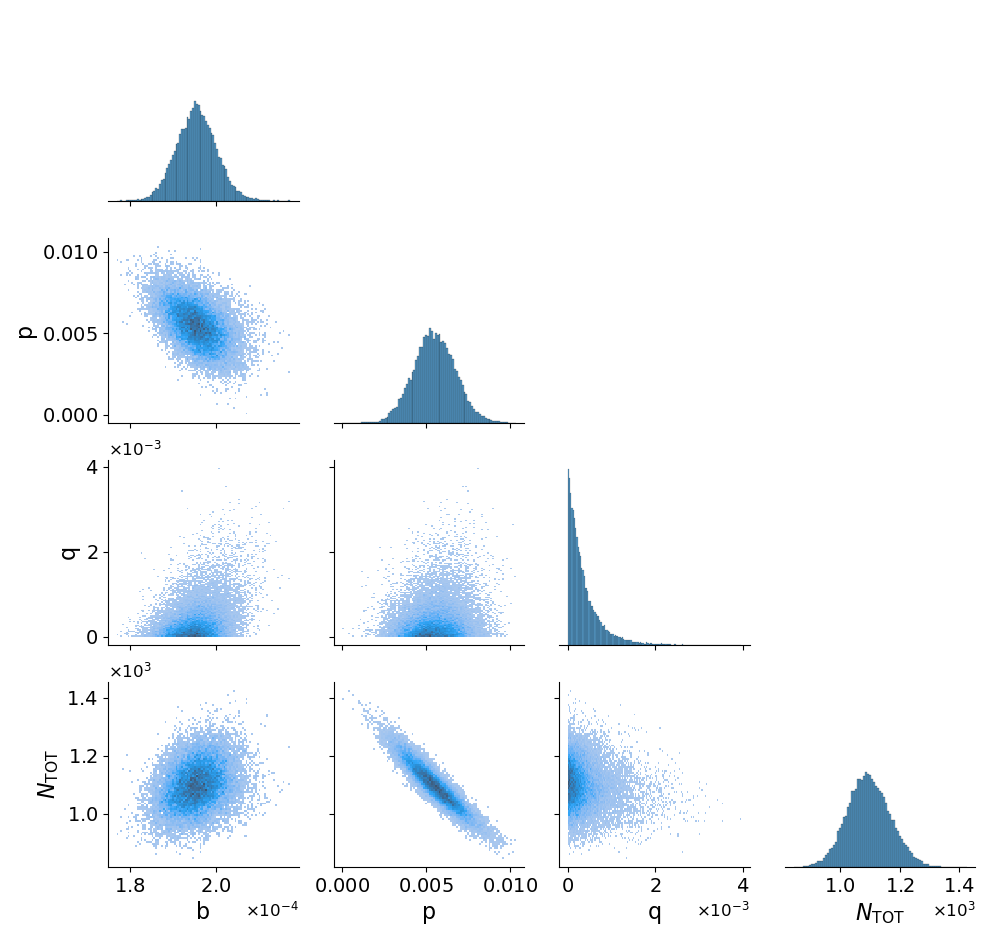}
\caption{Marginal and bivariate posterior distributions for the model parameters $\boldsymbol{\theta_M} = \{b,p,q,N_{\text{TOT}}\}$ when MCMC is used to fit model variant $\mathcal{M}_{3,1}$ to summary statistics $S_0(t),S_1(t),S_2(t)$ extracted from the invasive phenotype data.}
\label{fig:INV_shed_pairwise}
\end{figure}

\begin{figure}[H]
\centering
\includegraphics[width=\textwidth]{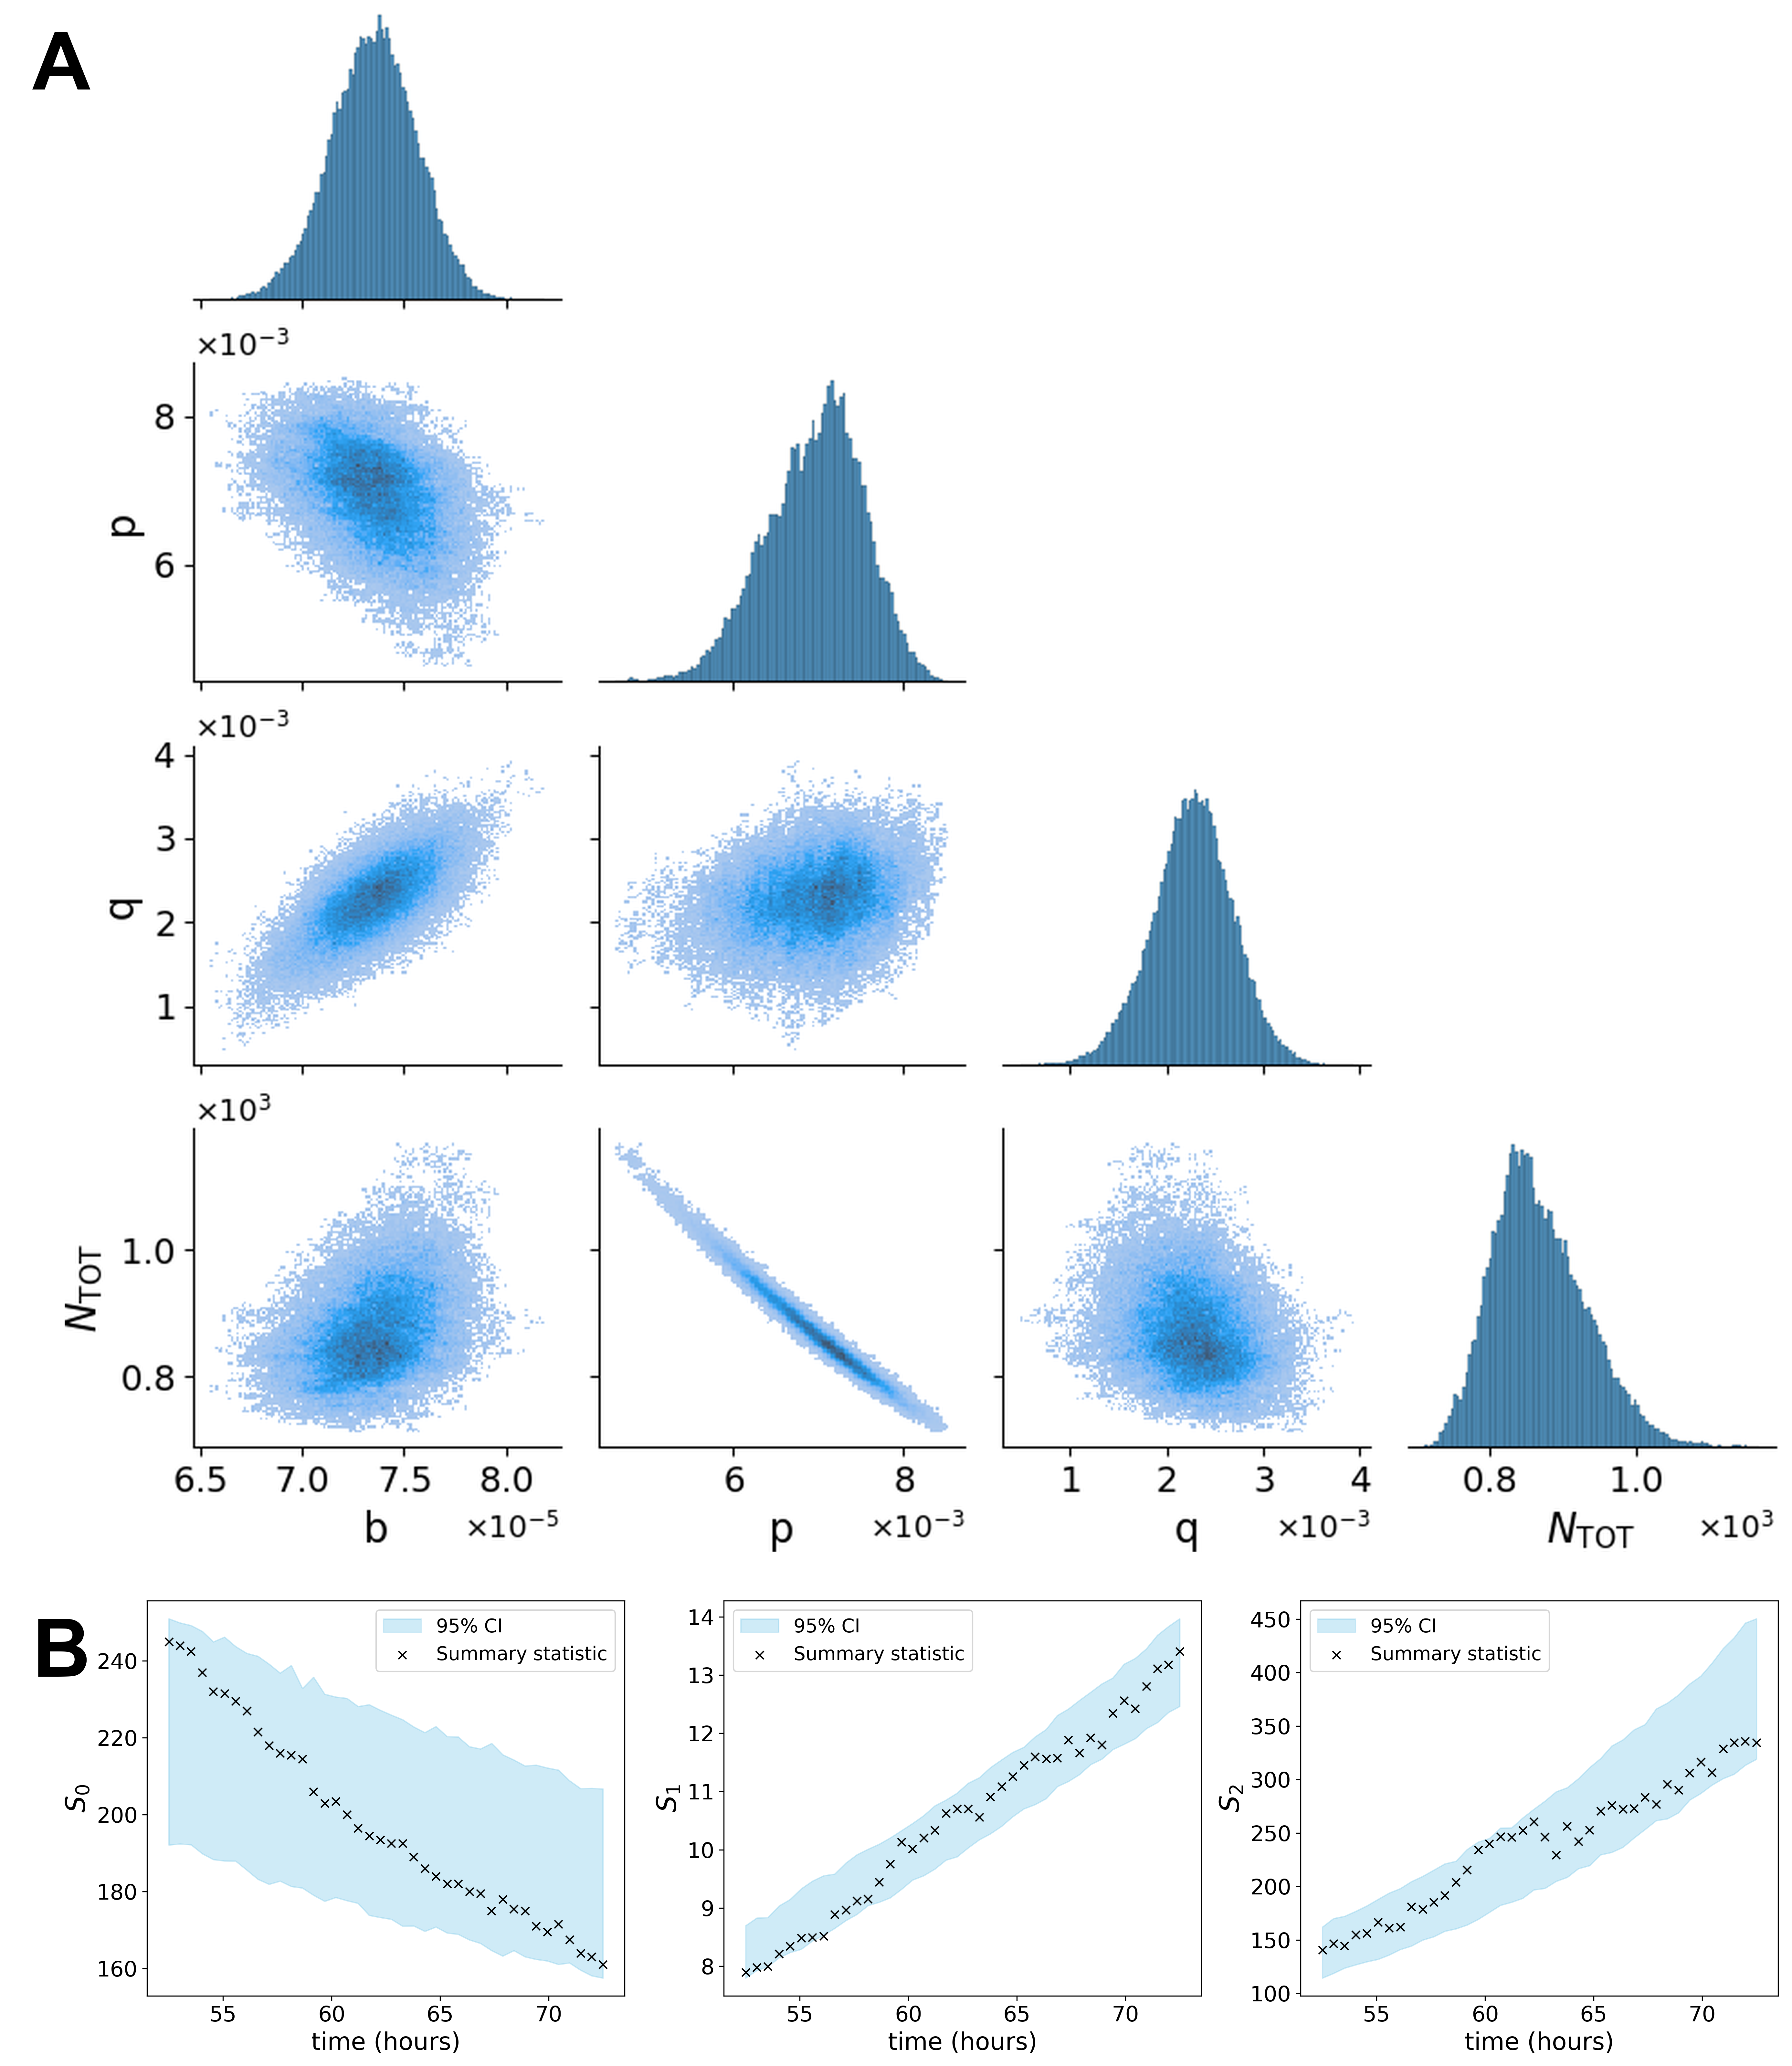}
\caption{MCMC plots for fitting model variant $\mathcal{M}_{3,1}$ to summary statistics $S_0(t),S_1(t),S_2(t)$ extracted from the proliferative phenotype data. (A) Marginal and bivariate posterior distributions for the model parameters $\boldsymbol{\theta_M} = \{b,p,N_{\text{TOT}}\}$. (B) Posterior predictive checks for the three summary statistics of the cluster size distribution.
Each subplot shows the summary statistic values (black crosses) over time alongside the $95\%$ prediction interval (red shaded region) generated from $1000$ posterior samples.}
\label{fig:PRO_MCMC_plots_cst_shed}
\end{figure}

\newpage

\begin{figure}[H]
\centering
\includegraphics[width=\textwidth]{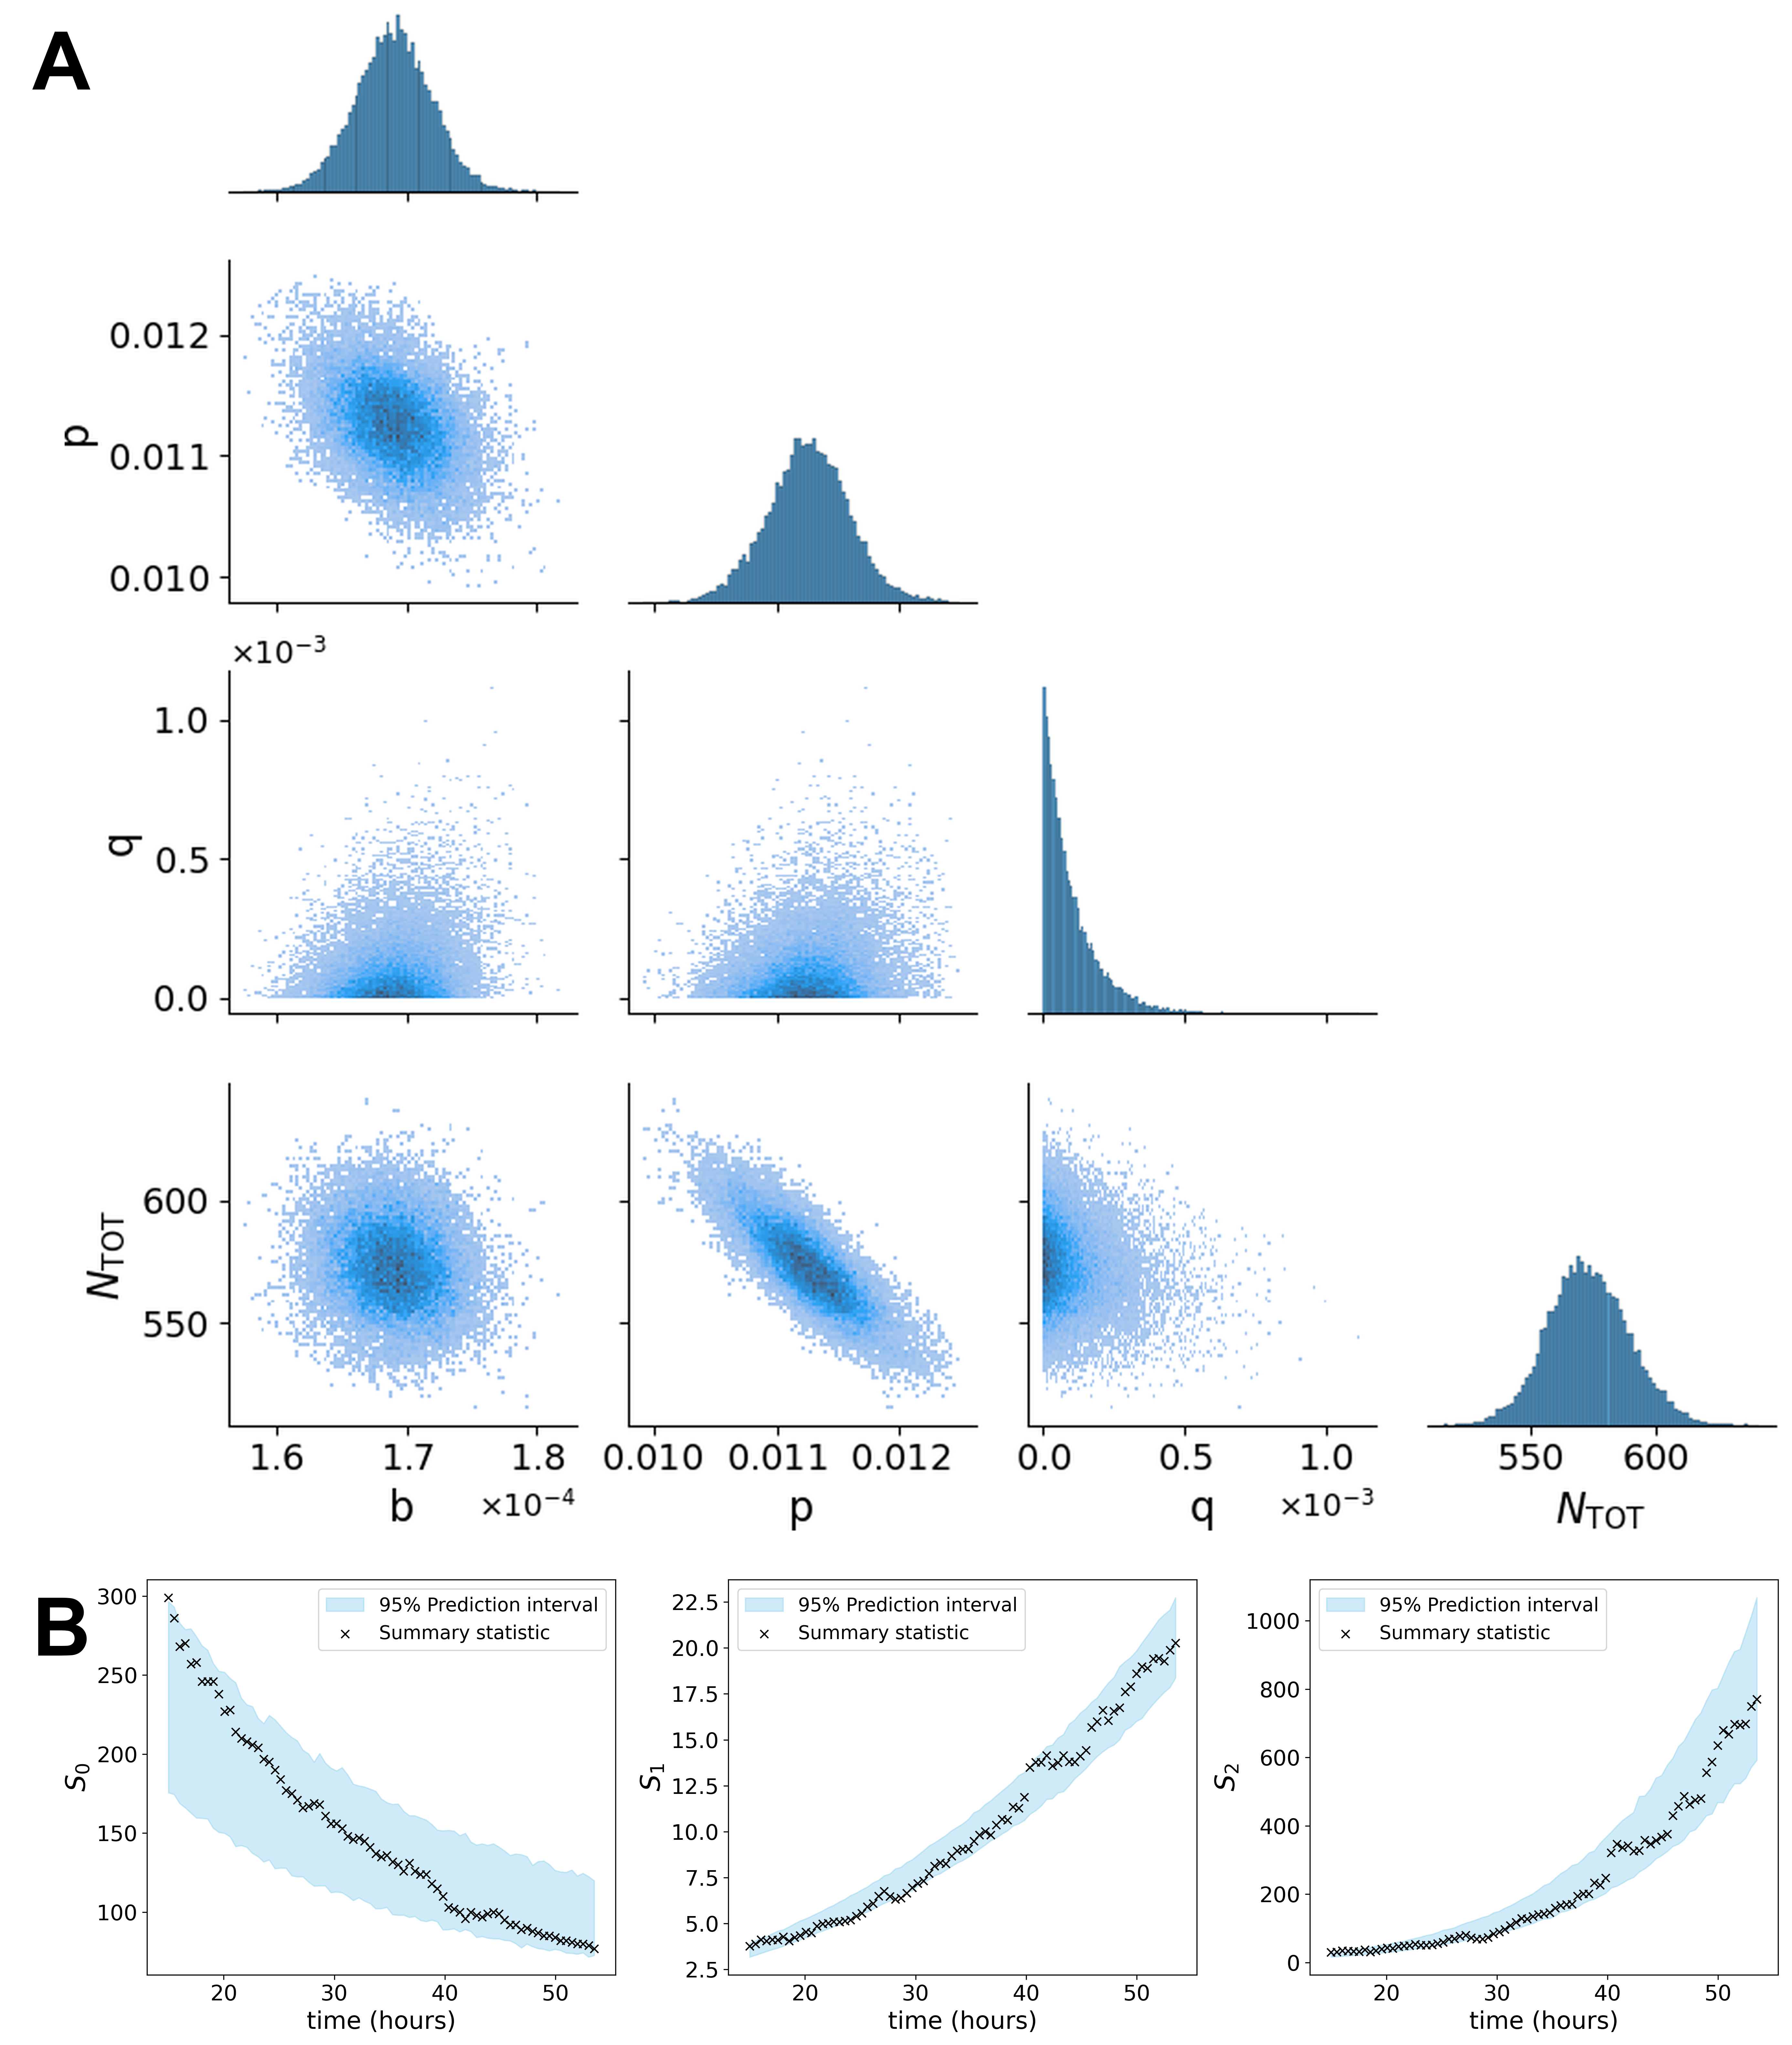}
\caption{MCMC plots for fitting model variant $\mathcal{M}_{3,1}$ to summary statistics $S_0(t),S_1(t),S_2(t)$ extracted from the co-cultured cell data. (A) Marginal and bivariate posterior distributions for the model parameters $\boldsymbol{\theta_M} = \{b,p,N_{\text{TOT}}\}$. (B) Posterior predictive checks for the three summary statistics of the cluster size distribution.
Each subplot shows the summary statistic values (black crosses) over time alongside the $95\%$ prediction interval (red shaded region) generated from $1000$ posterior samples.}
\label{fig:COMBO_MCMC_plots_cst_shed}
\end{figure}

\begin{figure}[H]
\centering
\includegraphics[width=\textwidth]{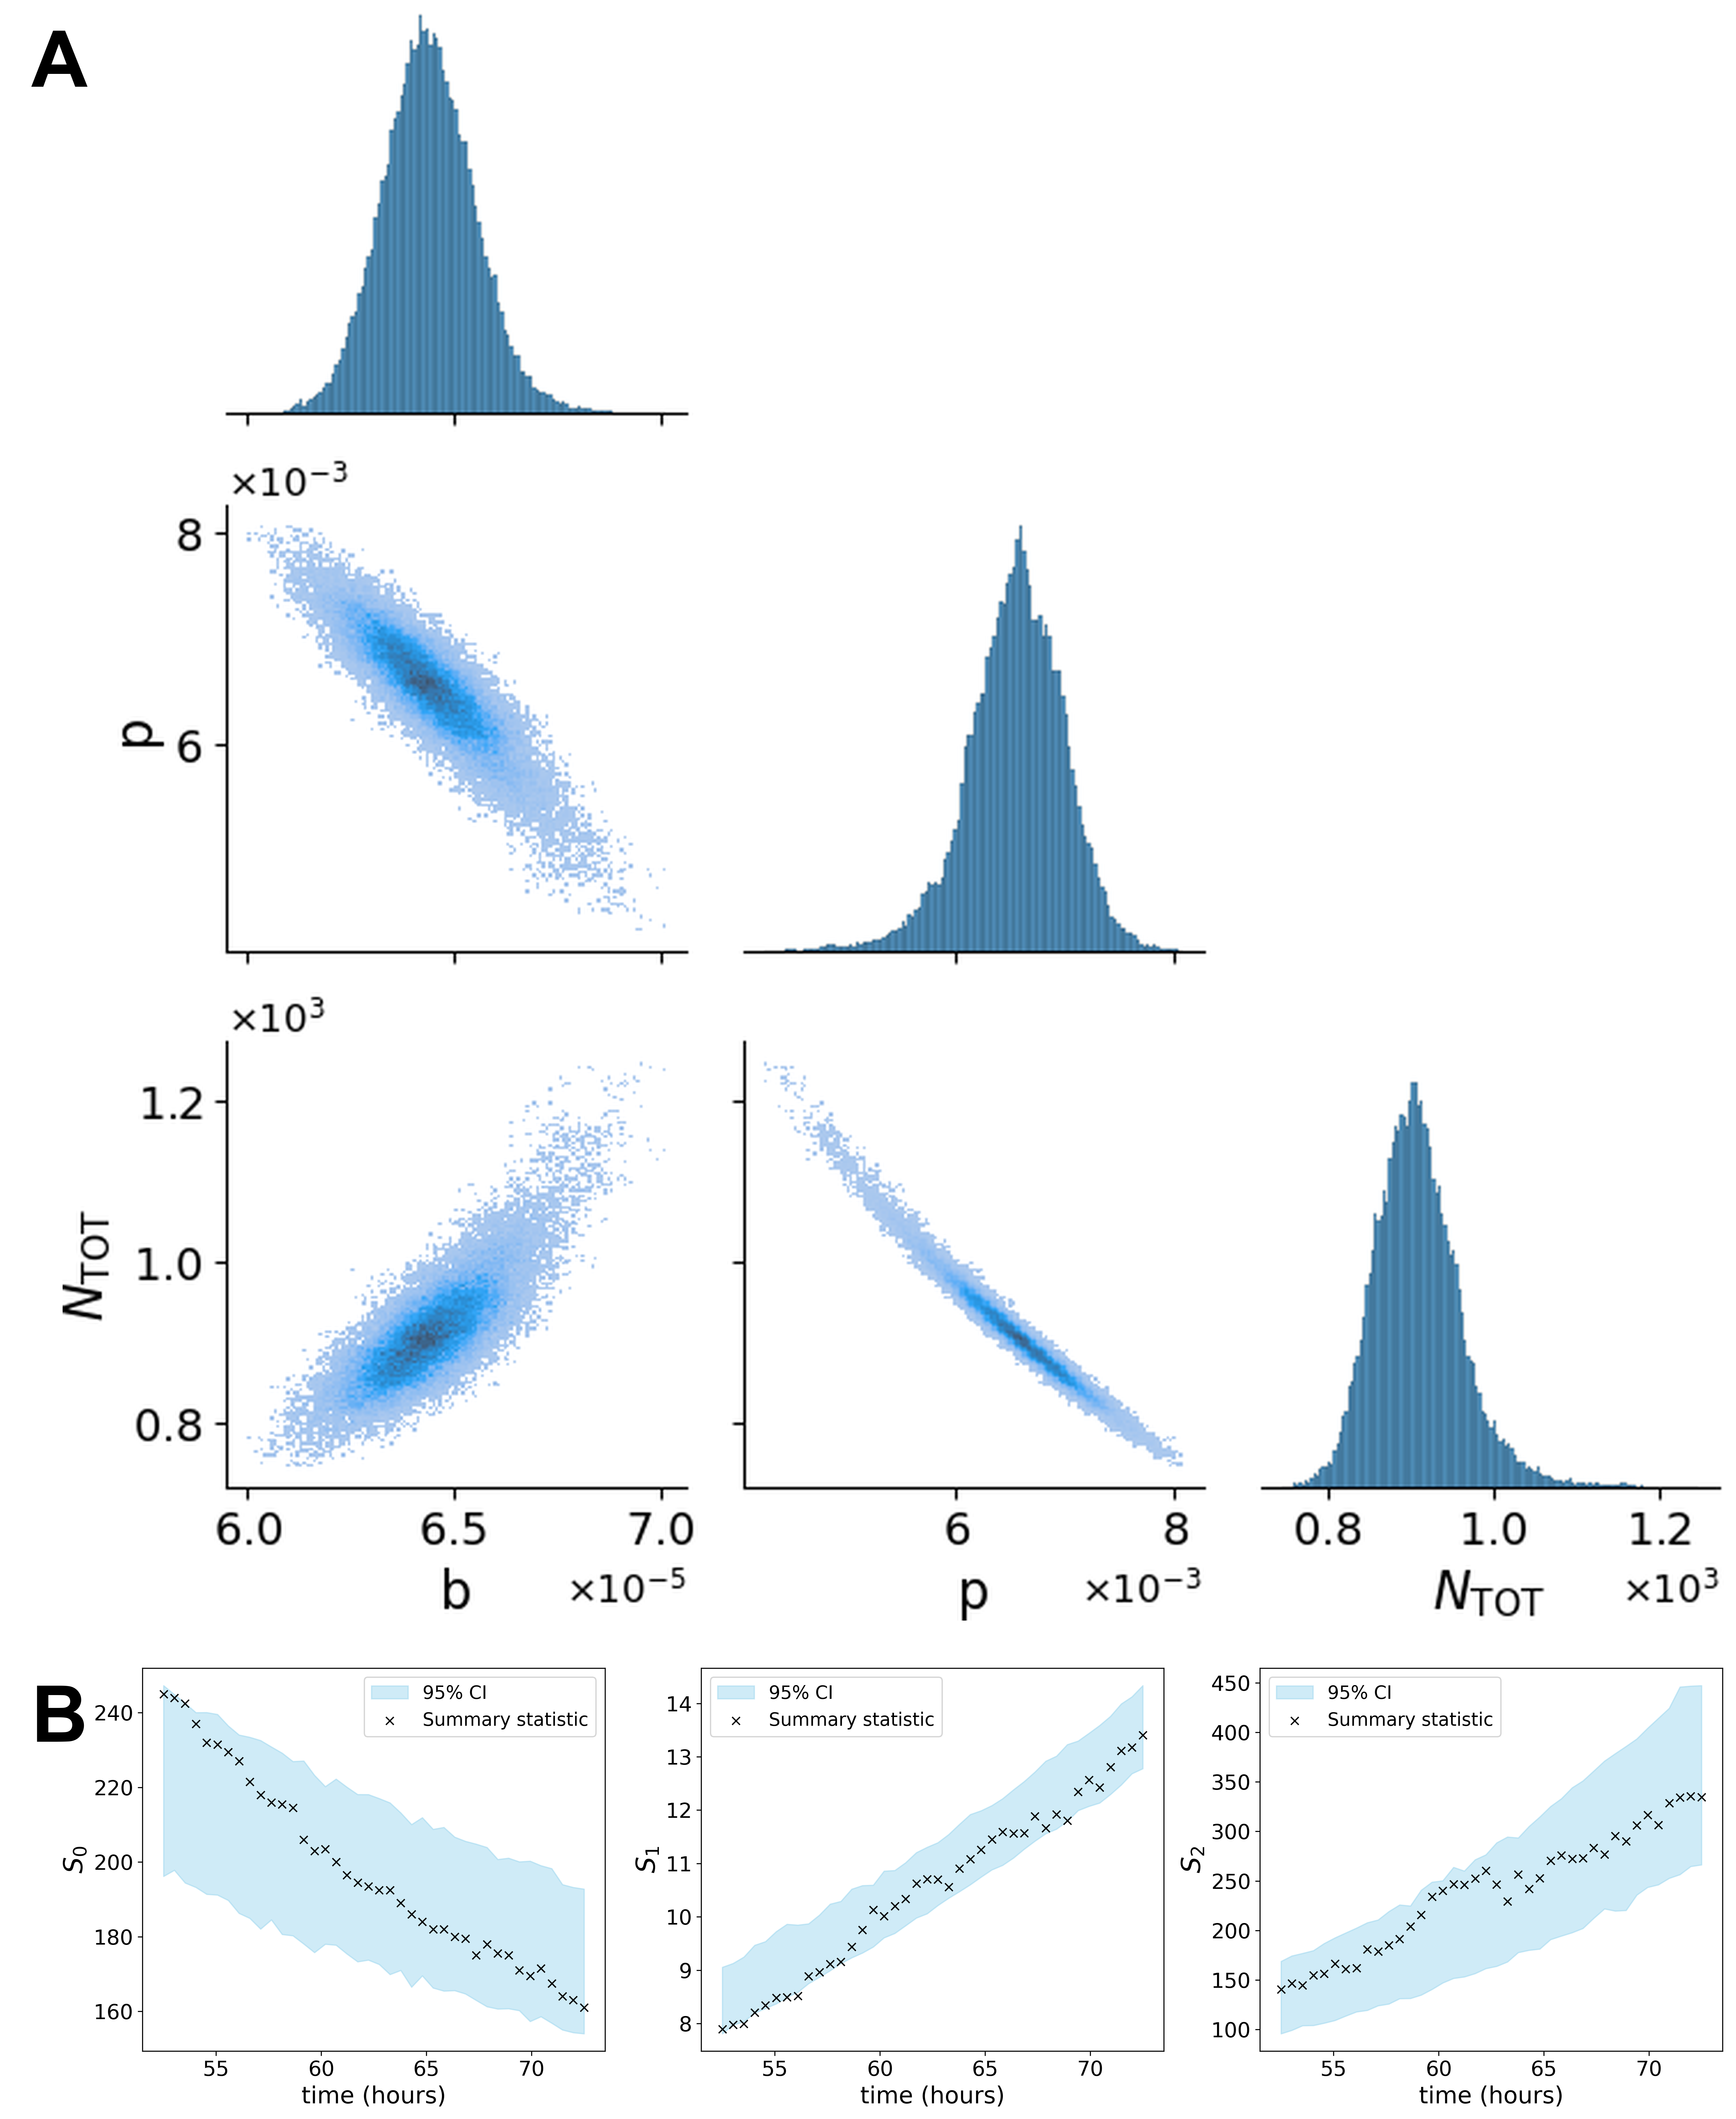}
\caption{MCMC plots for fitting model variant $\mathcal{M}_{3,0}$ to summary statistics $S_0(t),S_1(t),S_2(t)$ extracted from the proliferative phenotype data. (A) Marginal and bivariate posterior distributions for the model parameters $\boldsymbol{\theta_M} = \{b,p,N_{\text{TOT}}\}$. (B) Posterior predictive checks for the three summary statistics of the cluster size distribution.
Each subplot shows the summary statistic values (black crosses) over time alongside the $95\%$ prediction interval (red shaded region) generated from $1000$ posterior samples.}
\label{fig:PRO_MCMC_plots_no_shed}
\end{figure}

\begin{figure}[H]
\centering
\includegraphics[width=\textwidth]{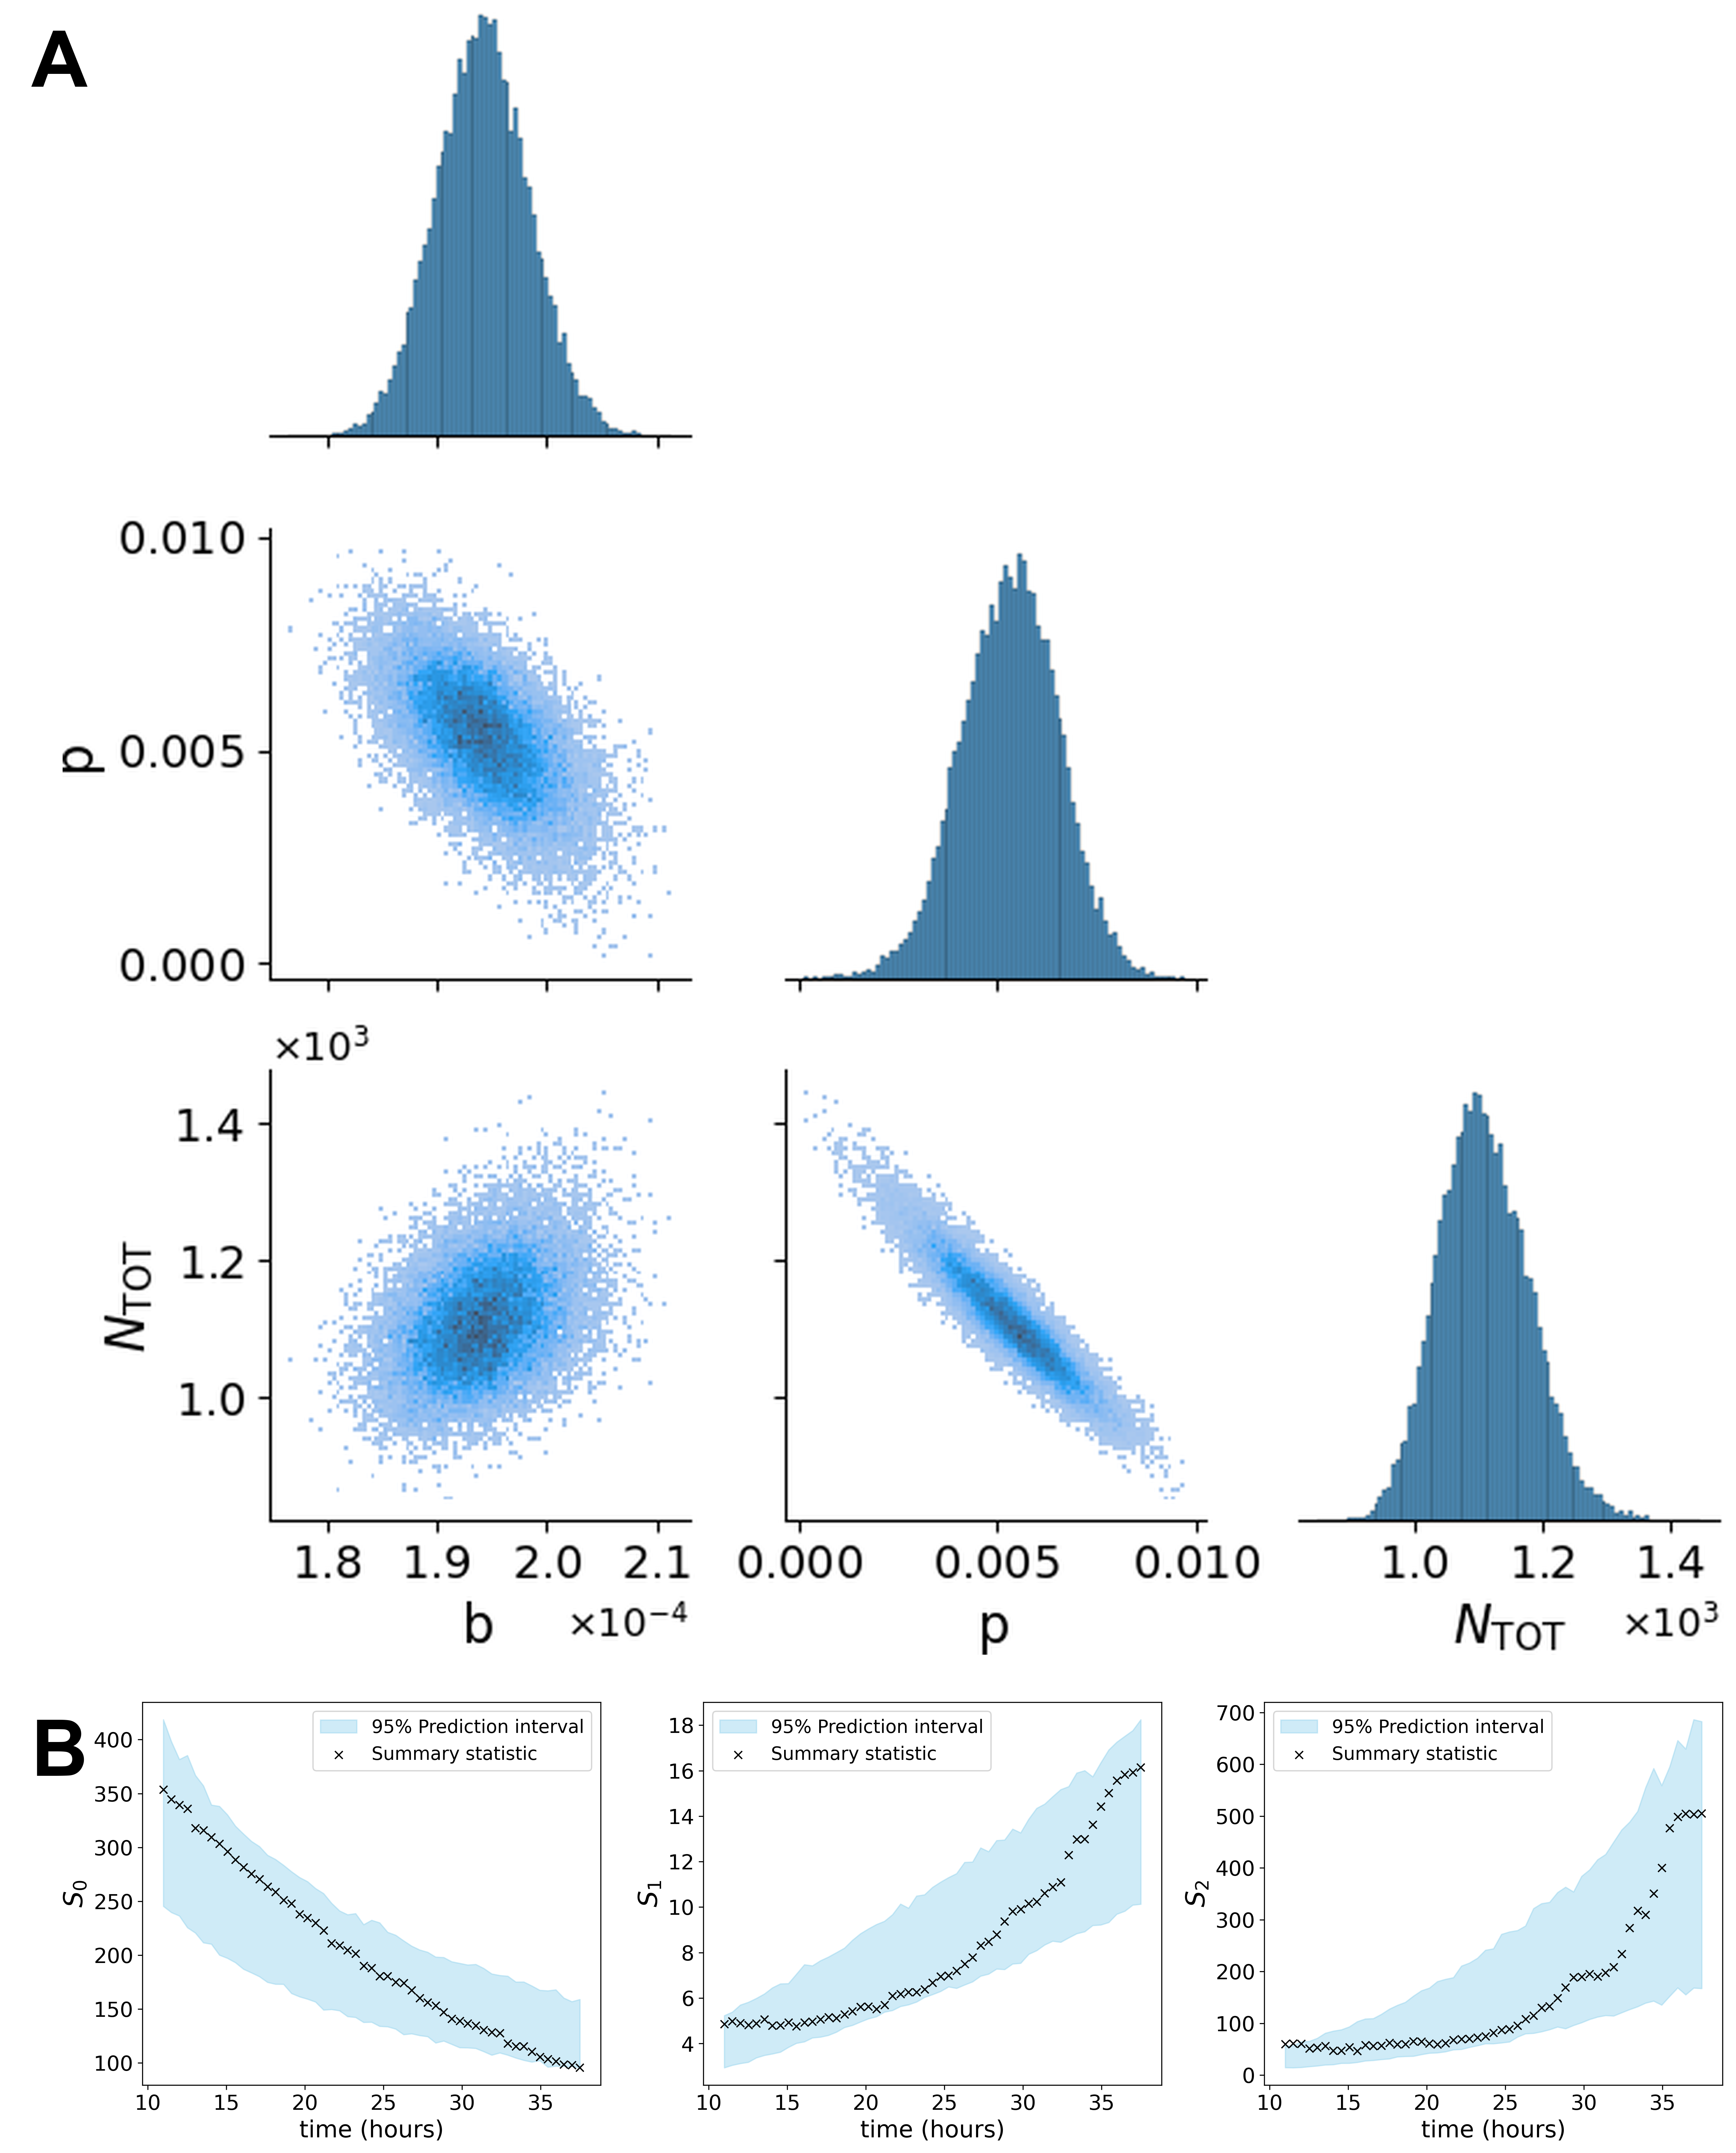}
\caption{MCMC plots for fitting model variant $\mathcal{M}_{3,0}$ to summary statistics $S_0(t),S_1(t),S_2(t)$ extracted from the invasive phenotype data. (A) Marginal and bivariate posterior distributions for the model parameters $\boldsymbol{\theta_M} = \{b,p,N_{\text{TOT}}\}$. (B) Posterior predictive checks for the three summary statistics of the cluster size distribution.
Each subplot shows the summary statistic values (black crosses) over time alongside the $95\%$ prediction interval (red shaded region) generated from $1000$ posterior samples.}
\label{fig:INV_MCMC_plots_no_shed}
\end{figure}

\begin{figure}[H]
\centering
\includegraphics[width=\textwidth]{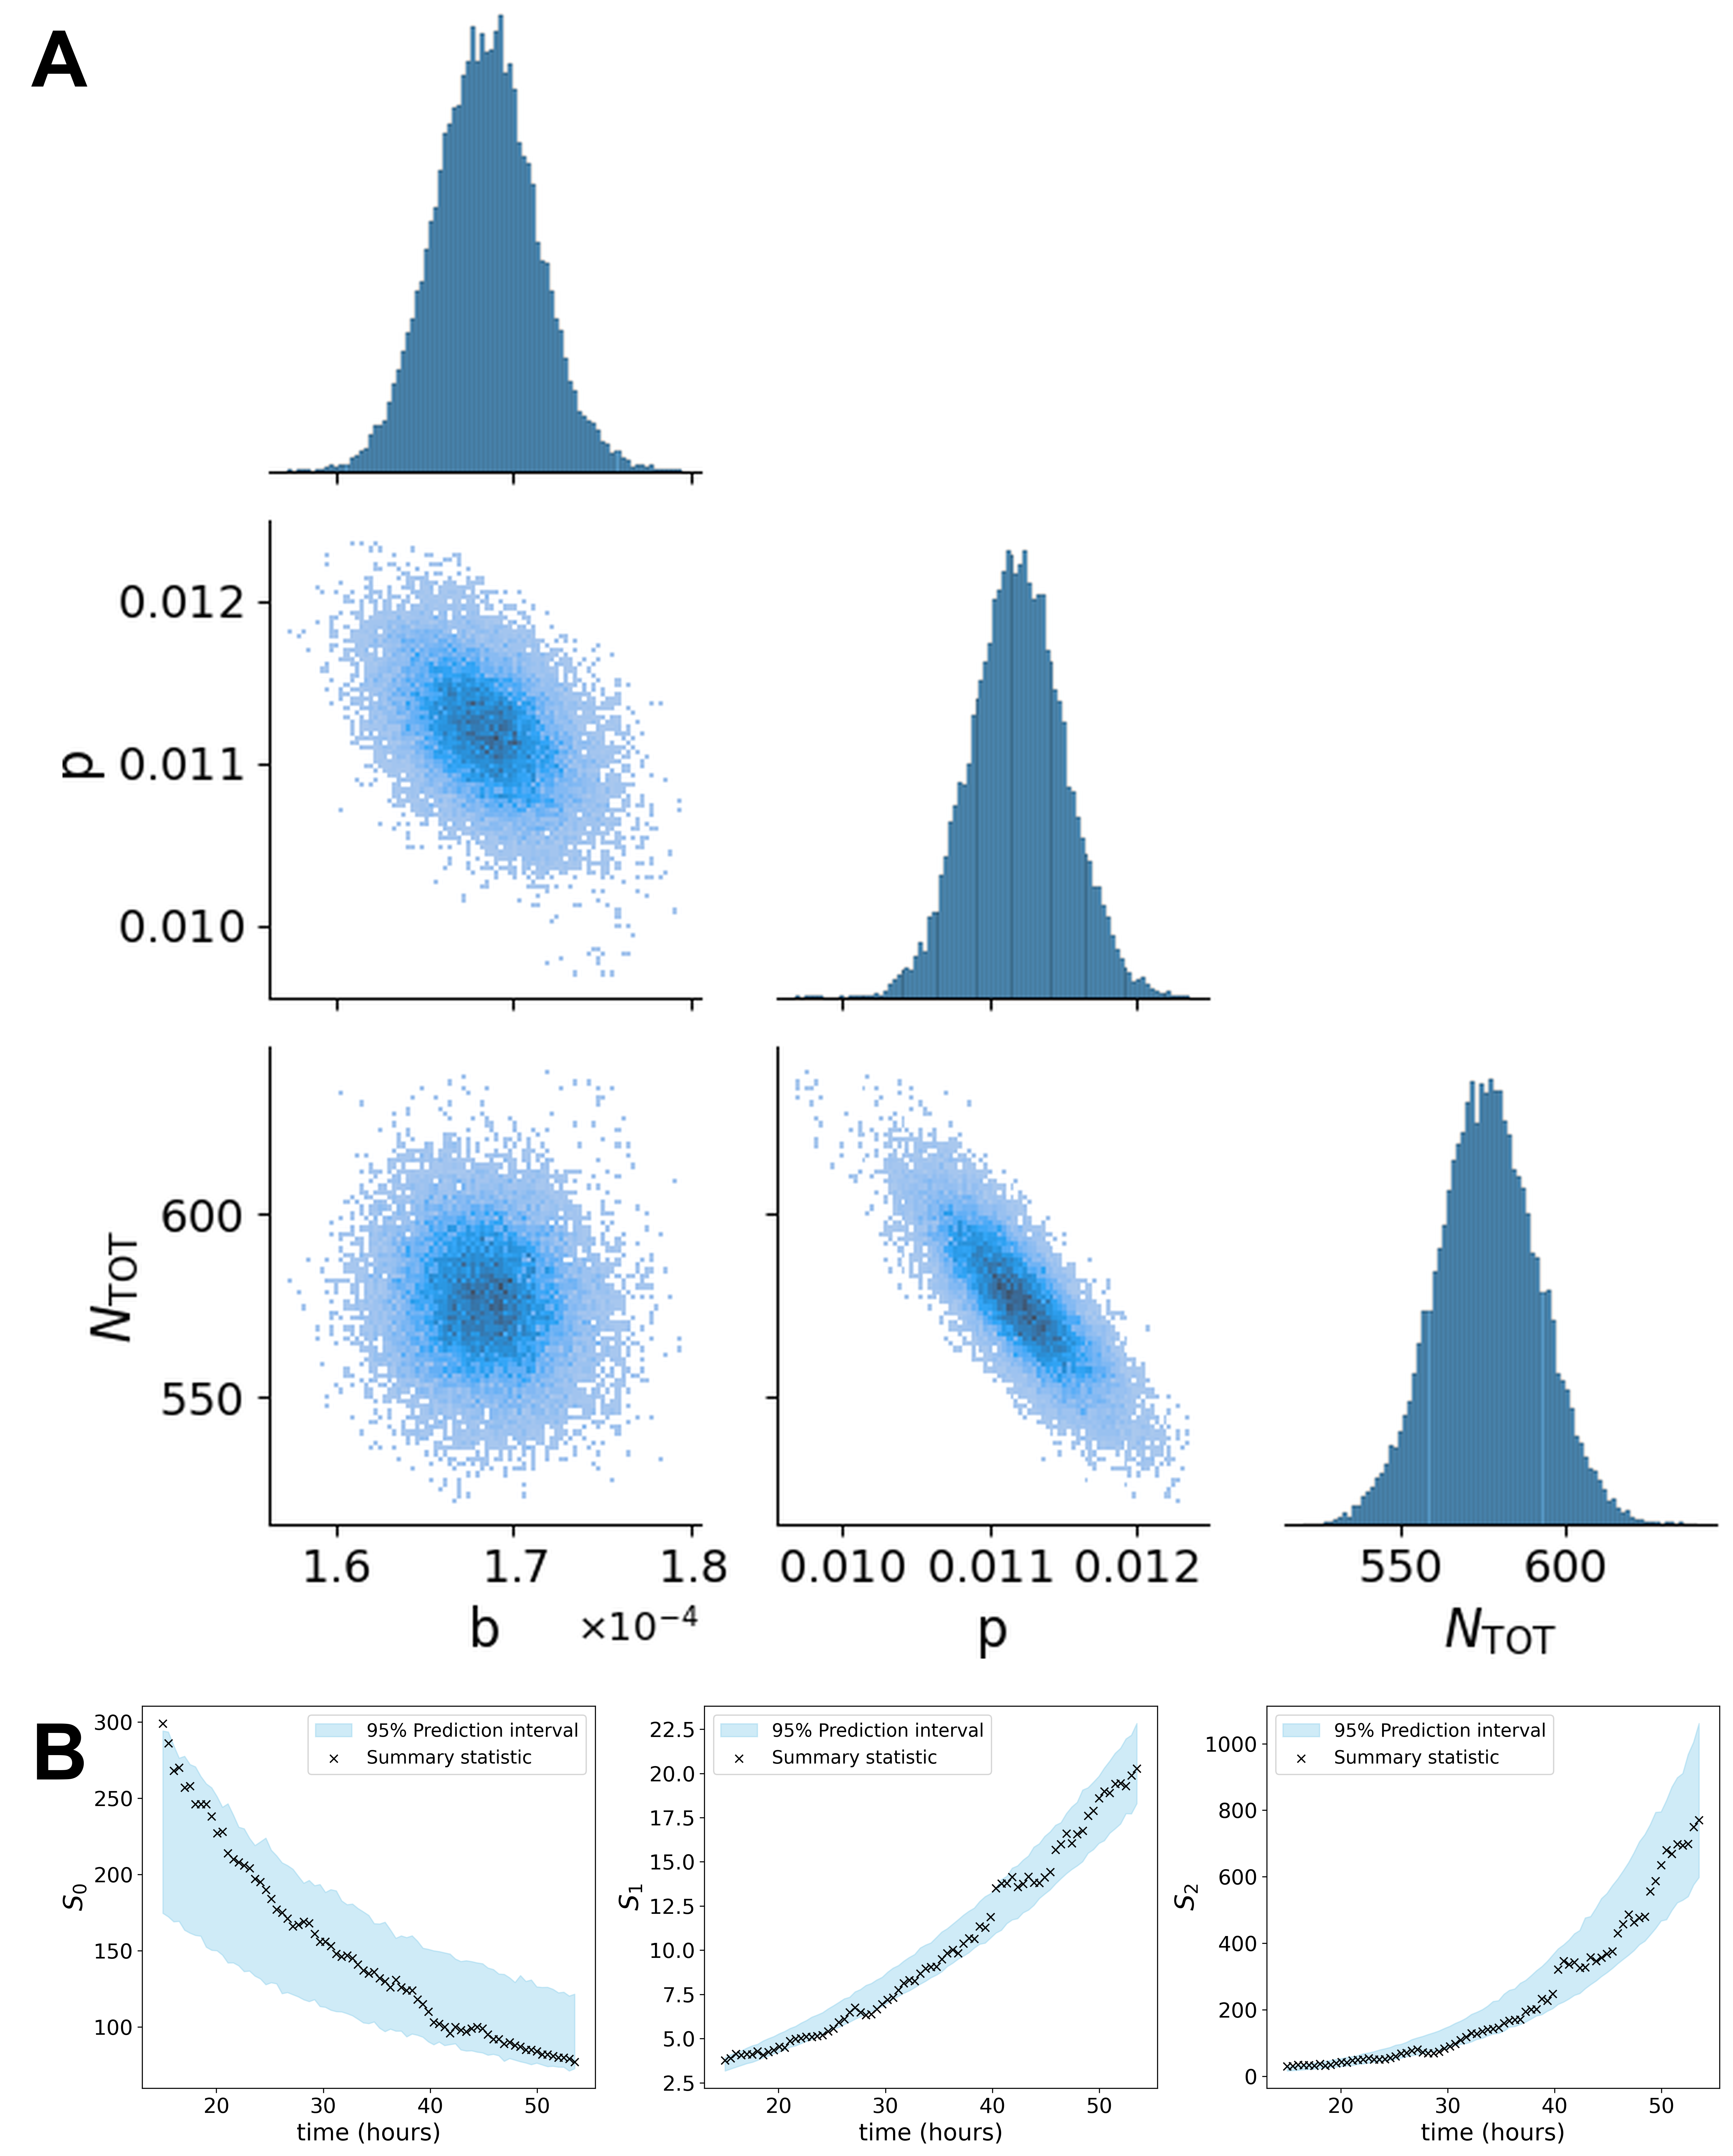}
\caption{MCMC plots for fitting model variant $\mathcal{M}_{3,0}$ to summary statistics $S_0(t),S_1(t),S_2(t)$ extracted from the co-cultured cell data. (A) Marginal and bivariate posterior distributions for the model parameters $\boldsymbol{\theta_M} = \{b,p,N_{\text{TOT}}\}$. (B) Posterior predictive checks for the three summary statistics of the cluster size distribution.
Each subplot shows the summary statistic values (black crosses) over time alongside the $95\%$ prediction interval (red shaded region) generated from $1000$ posterior samples.}
\label{fig:COMBO_MCMC_plots_no_shed}
\end{figure}

\subsubsection*{Model selection plots}
These figures show the $\Delta AIC$ values for each of the $16$ model variants when fitted to the invasive cell monoculture and co-cultured data in turn. This shows that the best performing model in both cases is model variant $\mathcal{M}_{3,0}$, which has proliferation proportional to the number of cells in a cluster and no shedding.

\begin{figure}[H]
\centering
\includegraphics[width=\textwidth]{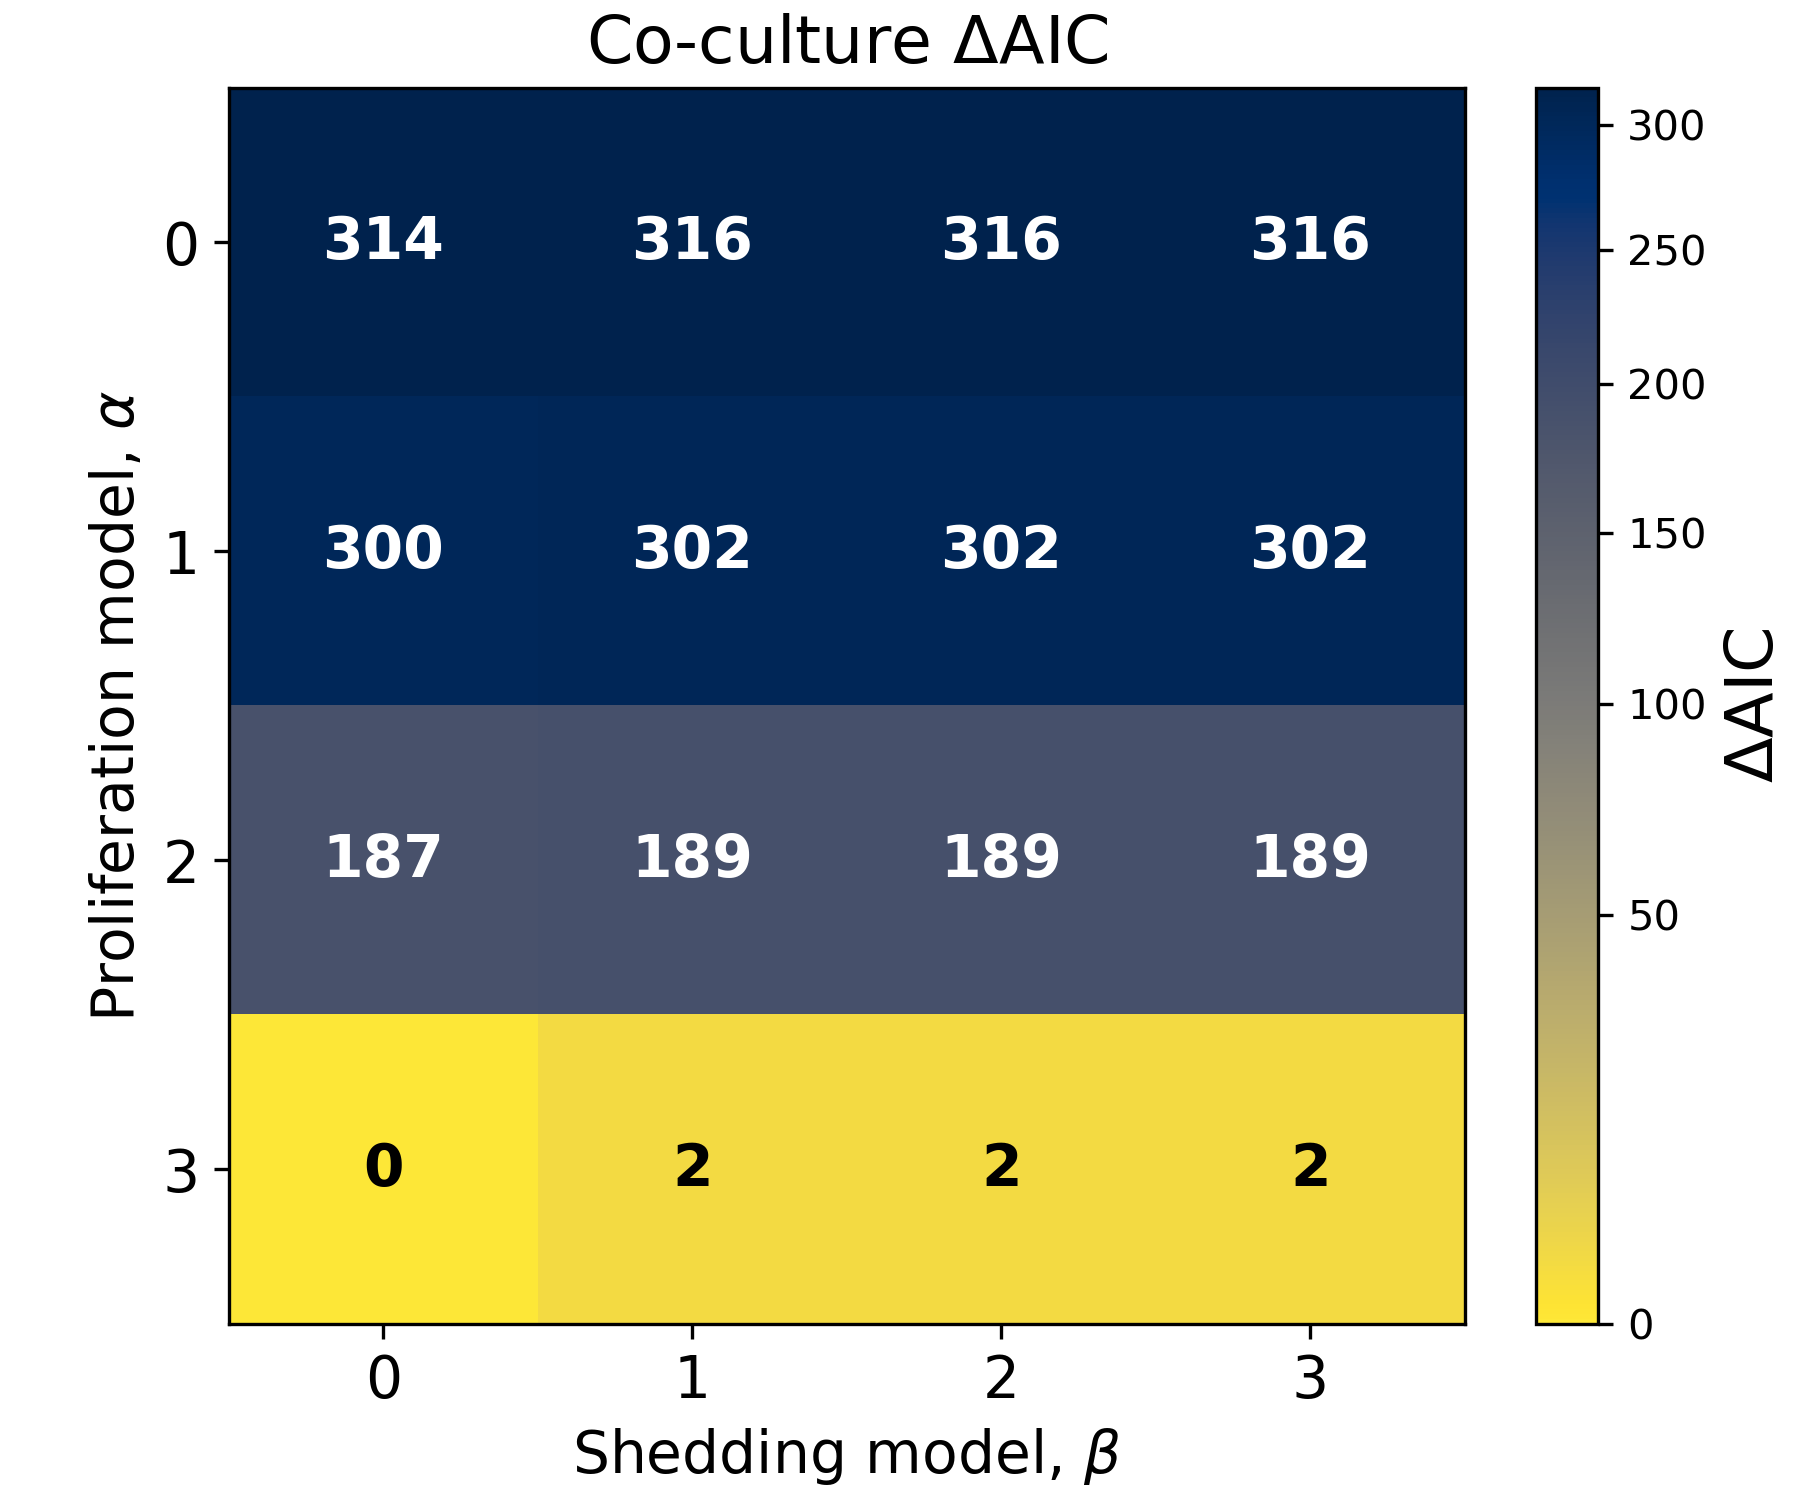}
\caption{$\Delta AIC$ values comparing different combinations of proliferation and shedding model variants for co-culture populations, assuming constant coagulation kernels. Each row corresponds to a different functional form for proliferation ($\alpha = 0$ for no proliferation, $\alpha = 1$ for constant proliferation, $\alpha = 2$ for surface area proliferation, and $\alpha = 3$ for cell number proliferation), while each column indicates the functional form for shedding $(\beta = 0,1,2,3)$. Lower $\Delta AIC$ values indicate better model performance.}
\label{fig:COMBO_AIC_values}
\end{figure}

\subsubsection*{Comparison between phenotypes}
Figure \ref{fig:PRO_INV_COMBO_Cell_num_cst_pairwise} shows parameter regimes for each experimental condition. It is the corresponding plot to Figure 5 of the main text when applied to model variant $\mathcal{M}_{3,1}$ rather than model variant $\mathcal{M}_{3,0}$. The co-culture coagulation parameter, $b$, appears between the values for the monocultures, whereas the proliferation rate, $p$, is greater in the co-culture than either of the monocultures, matching the behaviour of Figure 5. The shedding rate, $q$, for invasive phenotype cells and the co-culture is peaked at zero, which is the MLE value, and rapidly decays away from zero, whereas the unimodal, bell-shaped posterior distribution for the shedding parameter with the proliferative phenotype data is also evident.

\begin{figure}[H]
\centering
\includegraphics[width=\textwidth]{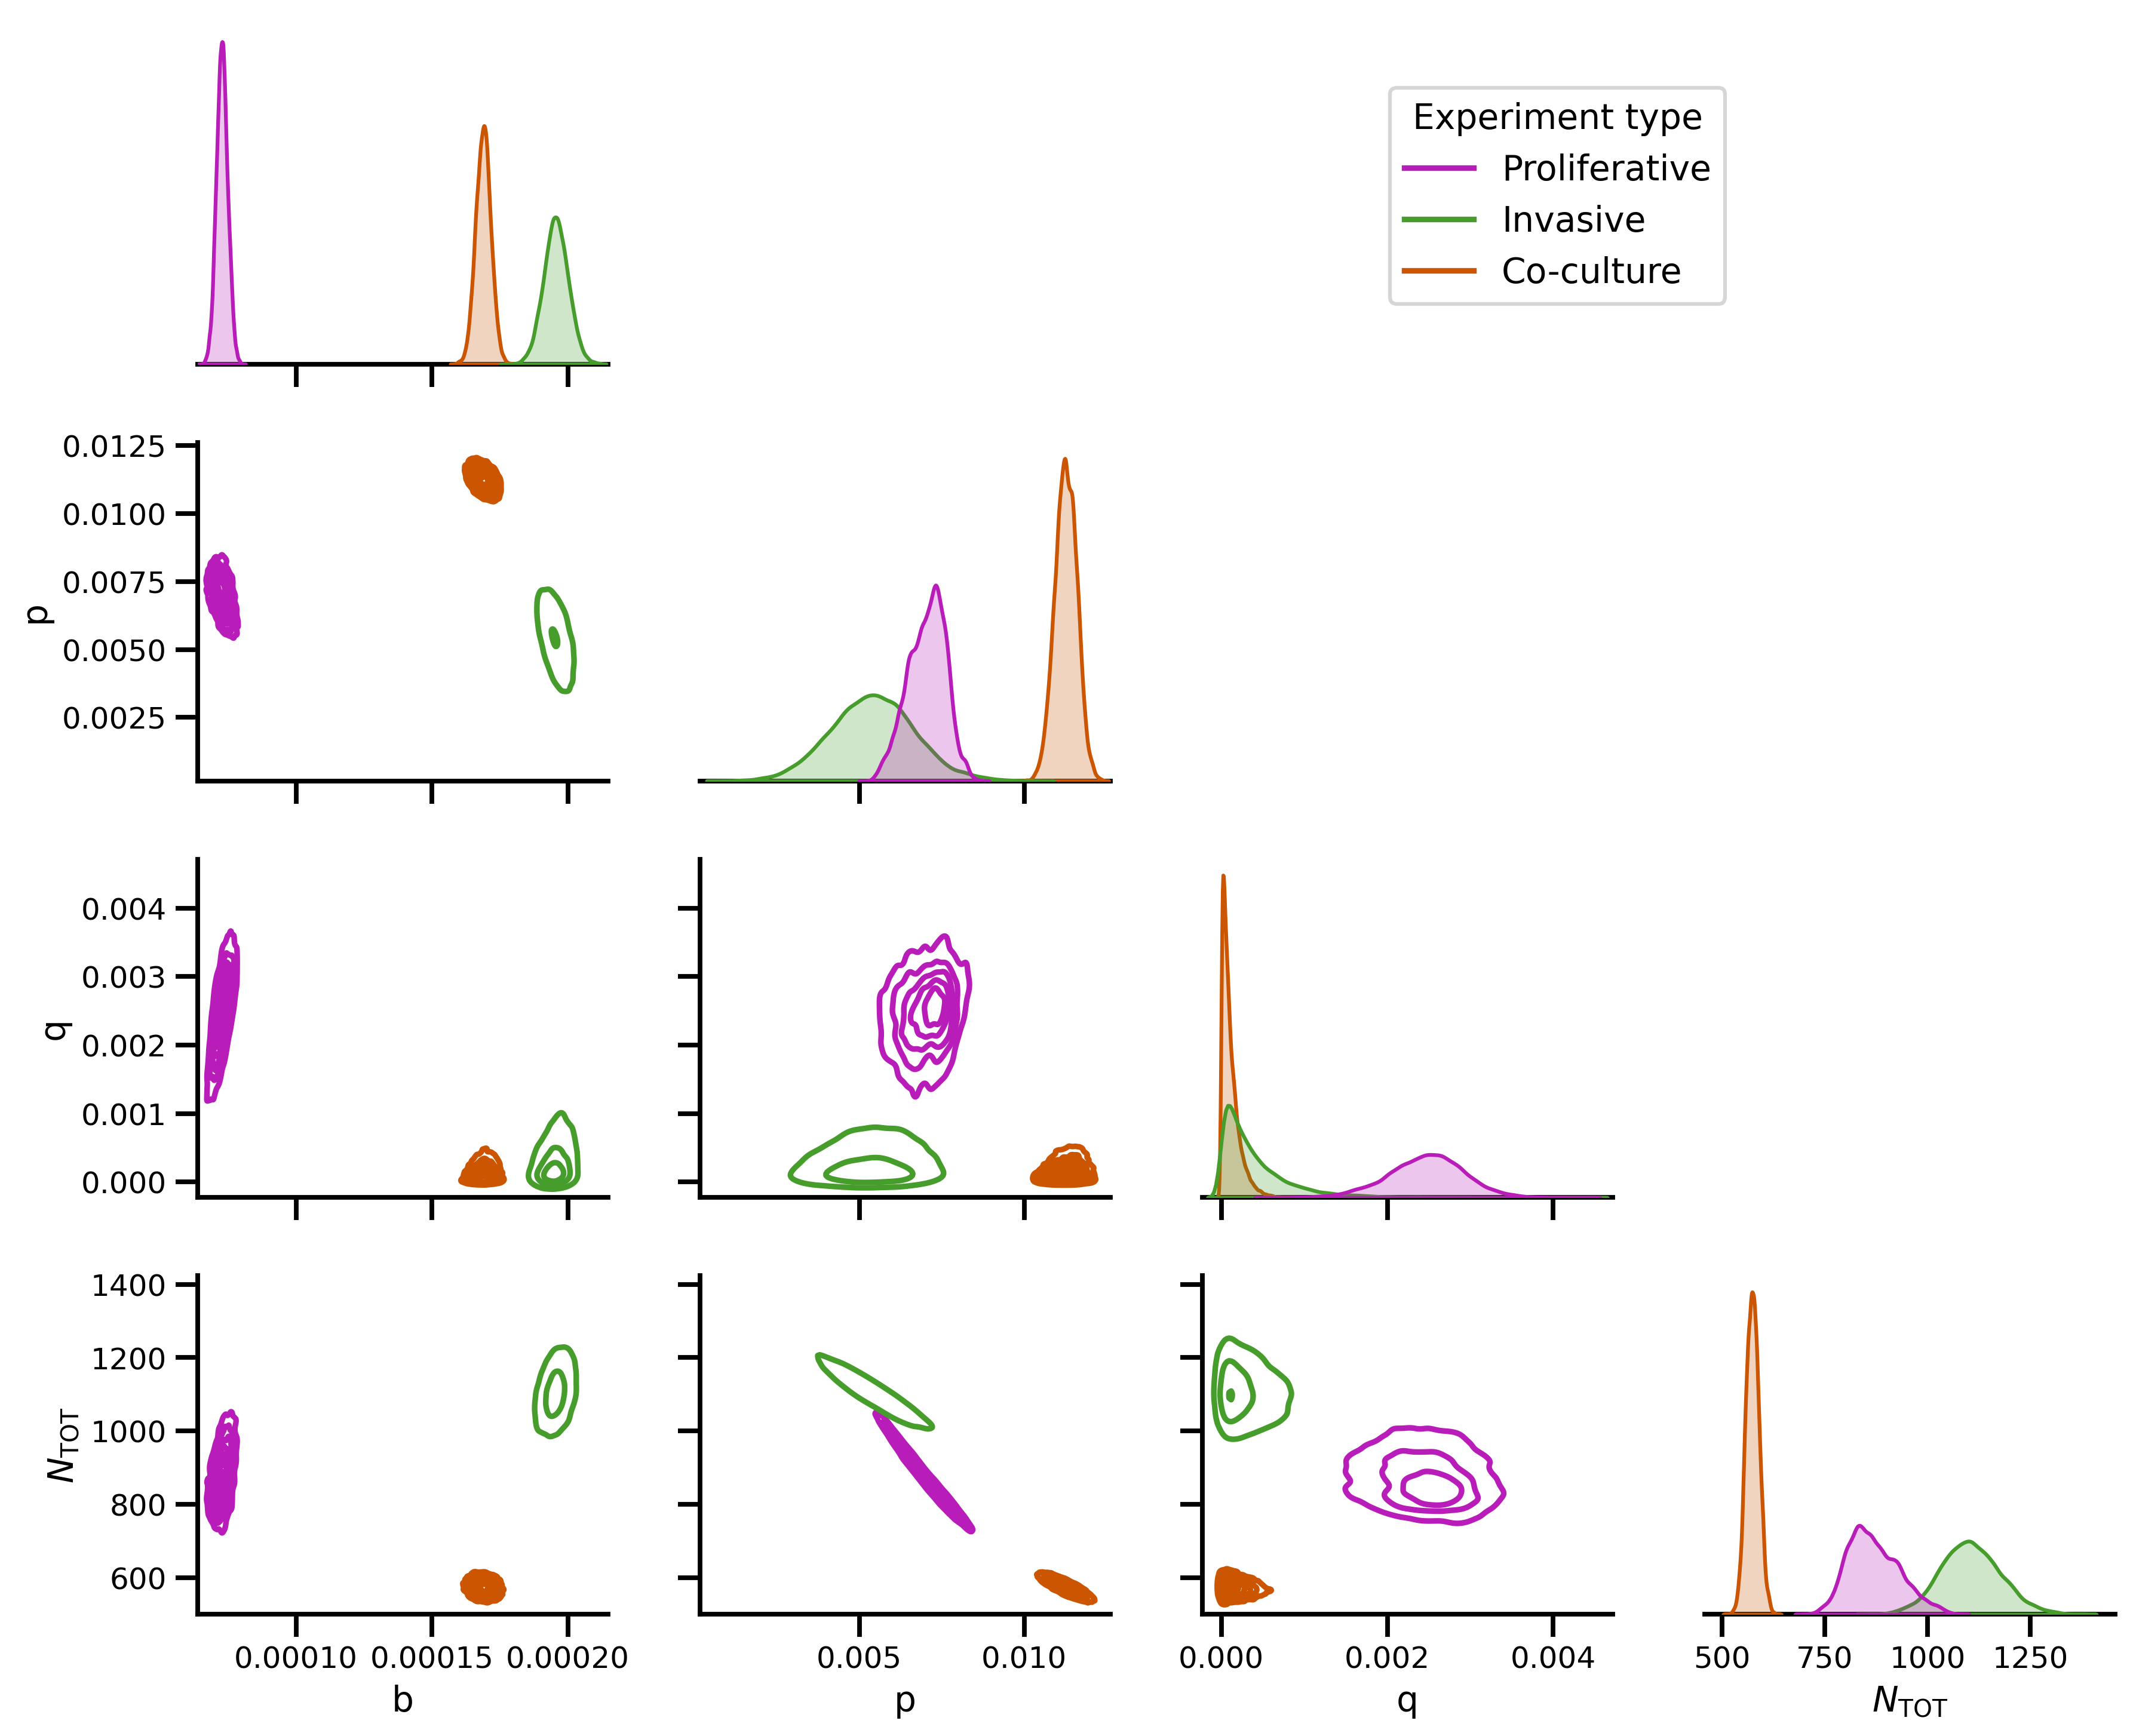}
\caption{Marginal and bivariate posterior distributions for model parameters $\boldsymbol{\theta_M} = \{b,p,q,N_{\text{TOT}}\}$ when model variant $\mathcal{M}_{3,1}$ is fitted to data for each of the three experimental types. Plots are coloured by the experiment type (proliferative: magenta, invasive: green, and co-culture: orange).}
\label{fig:PRO_INV_COMBO_Cell_num_cst_pairwise}
\end{figure}

\bibliography{paper-bibliography}

\end{document}
